# Supplementary material for: Testing for latent structure via the Wilcoxon--Wigner random matrix of normalized rank statistics
Source: arXiv:2512.18924 source file (2025-12-21)
Supplement: Supplementary file 1 [file supplement.pdf]

# Supplementary material for "Testing for latent structure via the Wilcoxon–Wigner random matrix of normalized rank statistics"

By Jonquil Z. Liao

*Department of Statistics, University of Wisconsin–Madison,*
*1205 University Avenue, Madison, Wisconsin 53706, U.S.A.*
zliao42@wisc.edu

Joshua Cape

*Department of Statistics, University of Wisconsin–Madison,*
*1205 University Avenue, Madison, Wisconsin 53706, U.S.A.*
jrcape@wisc.edu

## Overview

This document provides proofs of all the main results and additional discussion.

## Notation

Given a positive integer $l$, let $[\![l]\!] = \{1, \ldots, l\}$. Let $1_n$ denote the $n$-dimensional vector of all ones. Let $J$ denote the matrix of all ones, and let $I$ denote the identity matrix when the respective dimensions are understood from context. Let $\mathbb{I}\{\cdot\}$ denote the binary indicator function. Let $\|A\|$ denote the spectral norm of the matrix $A$. Let $\|A\|_{\mathrm{F}}$ denote the Frobenius norm of the matrix $A$. Let $C_b(\mathbb{R})$ denote the set of bounded continuous functions from $\mathbb{R}$ to $\mathbb{R}$, and let $\mathcal{B}$ denote the Borel $\sigma$-algebra on $\mathbb{R}$.

For asymptotic notation, $f(n) = O\{g(n)\}$ signifies that there exist positive constants $k$ and $n_0$ such that $|f(n)| \le kg(n)$ whenever $n \ge n_0$. Similarly, $f(n) = o\{g(n)\}$ signifies that for all $k > 0$, there exists a positive constant $n_0$ such that $|f(n)| \le kg(n)$ whenever $n \ge n_0$. In some contexts, with a slight abuse of notation, we write $f(n) = O\{g(n)\}$ to denote $f(n) = \Theta\{g(n)\}$, indicating both $f(n) = O\{g(n)\}$ and $g(n) = O\{f(n)\}$. Additionally, $f(n) \gg g(n)$ signifies that $\lim_{n\to\infty} |f(n)/g(n)| = \infty$. Regarding notation for asymptotic probability statements, $f(n) = O_p\{g(n)\}$ signifies that for any $\epsilon > 0$, there exist positive constants $k_\epsilon$ and $N_\epsilon$ such that $\mathrm{pr}\{|f(n)| \ge k_\epsilon g(n)\} \le \epsilon$ holds for all $n \ge N_\epsilon$. Similarly, $f(n) = o_p\{g(n)\}$ signifies that for any $k > 0$ it holds that $\lim_{n\to\infty} \mathrm{pr}\{|f(n)| \ge kg(n)\} = 0$.

Let $\mathrm{vech}_0(A)$ denote the half-vectorization of a given symmetric matrix $A \in \mathbb{R}^{n\times n}$, excluding the main diagonal. Given a set $S$, let $|S|$ denote the cardinality of $S$. Let $\mathfrak{i}$ denote the unit imaginary number satisfying $\mathfrak{i}^2 = -1$.

PROOF INGREDIENTS

Given two cumulative distribution functions $F^A$ and $F^B$, the Lévy distance between them is defined as

$$L(F^A, F^B) = \inf\left\{\varepsilon > 0 : F^A(x-\varepsilon) - \varepsilon \le F^B(x) \le F^A(x+\varepsilon) + \varepsilon, \text{ for all } x \in \mathbb{R}\right\}.$$

LEMMA 1. *Let $A$ and $B$ be two $n \times n$ real-valued symmetric matrices (hence normal matrices) with empirical spectral distributions $F^A$ and $F^B$, respectively. Then,*

$$L^3(F^A, F^B) \le \frac{1}{n}\|A - B\|_{\mathrm{F}}^2,$$

*where $L^3(F^A, F^B)$ denotes the third power of $L(F^A, F^B)$.*

LEMMA 2. *Let $P$ and $P_n$ for all $n \ge 1$ be probability measures on $(\mathbb{R}, \mathcal{B})$ with corresponding cumulative distribution functions $F$ and $F_n$, respectively. The following statements are equivalent:*

$$\lim_{n\to\infty} \int_{\mathbb{R}} f \, \mathrm{d}P_n = \int_{\mathbb{R}} f \, \mathrm{d}P \text{ for all } f \in C_b(\mathbb{R}); \tag{a}$$

$$\lim_{n\to\infty} F_n(x) = F(x) \text{ for every continuity point } x \text{ of } F; \tag{b}$$

$$\lim_{n\to\infty} L(F_n, F) = 0. \tag{c}$$

Next, we state several key technical lemmas which are proved further below.

LEMMA 3. *Let $n \ge 2$, and write $N = n(n-1)/2$. Let $a_1, \ldots, a_N$ be independent random variables from absolutely continuous distributions $F_1, \ldots, F_N$, respectively. For each $1 \le i \le N$, let $R_i$ denote the corresponding rank statistic of $a_i$, and let $\Gamma_i$ denote the centered, normalized rank statistic $\{R_i - E(R_i)\}/(N+1)$. Let $l, \delta_1, \ldots, \delta_l$ be arbitrary fixed positive integers, and let $1 \le i_1, \ldots, i_l \le N$ be $l$ distinct positive integers. Then,*

$$\left|E(\Gamma_{i_1}^{\delta_1}\Gamma_{i_2}^{\delta_2}\cdots\Gamma_{i_l}^{\delta_l}) - E(\Gamma_{i_1}^{\delta_1})E(\Gamma_{i_2}^{\delta_2})\cdots E(\Gamma_{i_l}^{\delta_l})\right| = O(N^{-1}).$$

LEMMA 4. *Assume the setting and notation in Lemma 3. Further define $m = |\{t \in \{1, \ldots, l\} : \delta_t = 1\}|$. Then, there exists a constant $C \equiv C(\delta_1 + \cdots + \delta_l) > 0$, such that*

$$\left|E(\Gamma_{i_1}^{\delta_1}\Gamma_{i_2}^{\delta_2}\cdots\Gamma_{i_l}^{\delta_l})\right| \le CN^{-m/2}.$$

LEMMA 5. *Assume the setting and notation in Lemma 3. Let $\Gamma \in \mathbb{R}^{n\times n}$ denote the symmetric matrix of centered normalized rank statistics where $\mathrm{vech}_0(\Gamma) = (\Gamma_1, \ldots, \Gamma_N)^{\mathrm{T}}$ and $\mathrm{diag}(\Gamma) = 0_{n\times n}$. Let $x$ and $y$ be arbitrary $n$-dimensional unit vectors. For any positive integer $l \ge 1$, it holds that*

$$E(x^{\mathrm{T}}\Gamma^l y) = \begin{cases} O(n^{l/2}) & \text{when } l \text{ is even,} \\ O\{n^{(l-1)/2}\} & \text{when } l \text{ is odd.} \end{cases}$$

LEMMA 6. *Assume the setting and notation in Lemma 5. For any positive integer $l \ge 1$,*

$$x^{\mathrm{T}}\{\Gamma^l - E(\Gamma^l)\}y = O_p\{n^{(l-1)/2}\}.$$

LEMMA 7. *Assume the setting and notation in Lemma 5. There exists a universal constant $C_1 > 0$ such that for all $n \ge 2$,*

$$\mathrm{pr}\left(\|\Gamma\| \ge 6n^{1/2}\right) \le \exp(-C_1 n).$$

Strictly speaking, Theorem 2 in the main text is a special case of Lemma 7. For context, we write "theorem" for Theorem 2 given its focal role in the main text, whereas we write "lemma" for Lemma 7 given its supporting role towards establishing theoretical guarantees for statistical hypothesis testing here in the supplement.

LEMMA 8. *Let $\Gamma$ be the (homogeneous) perturbation matrix defined in Eq. (2) in the main text. Write $\widetilde{\sigma}_n^2 = 8\sigma_n^4 n^{-1}$, where $\sigma_n^2 = 1/12 - 1/\{6(N+1)\}$ and $N = n(n-1)/2$. Let $u_1 = n^{-1/2}1_n$. Then, as $n \to \infty$, it holds that*

$$\frac{2\widetilde{\sigma}_n^{-1}}{n-1}\left(u_1^{\mathrm{T}}\Gamma^2 u_1 - \frac{n-1}{12}\right) \to N(0,1) \qquad \text{in distribution.}$$

## PROOFS OF MAIN RESULTS

Our overall proof strategy involves constructing first and second-order approximations for relevant quantities, such as linear forms of the leading eigenvector via $x^{\mathrm{T}}\{\Gamma^l - E(\Gamma^l)\}y$ for $l \geq 1$ with deterministic vectors $x, y$, and then establishing asymptotic normality of the dominant terms. The proof techniques used herein modify those for analyzing independent-entry noise models in Athreya et al. (2022); Fan et al. (2022) which leverage both the classical and martingale central limit theorems. In particular, the Wilcoxon–Wigner random matrix introduces additional complications due to the entrywise dependence among the normalized rank statistics and requires a different approach for establishing asymptotic normality. Notably, for the leading eigenvector $u_1 = n^{-1/2}1_n$, direct computation yields $u_1^{\mathrm{T}}\Gamma u_1 = 0$, making a first-order approximation inadequate. Instead, we develop perturbation expansions involving the dominating second-order term $u_1^{\mathrm{T}}\Gamma^2 u_1$ and then establish asymptotic normality by the moment matching method.

*Proof of Theorem 1.* Per the main text, let $A_{ij}$ for $1 \leq i < j \leq n$ be a random sample from an absolutely continuous distribution $F$. Let $A$ denote the hollow symmetric matrix whose strictly upper triangular entries are given by $\{A_{ij} : i < j\}$. Now, let $F(A) \in \mathbb{R}^{n\times n}$ denote the entry-wise application of the function $F$ to the matrix $A$, excluding the diagonal which is defined to be zero. By the probability integral transform, it follows that $\{F(A_{ij})\}_{i<j}$ is a random sample from $\mathrm{Unif}(0,1)$. Next, as in Eq. (2) of the main text, denote the residual matrix by $\Gamma = \widetilde{R} - 2^{-1}(J - I)$. This proof proceeds by decomposing $\Gamma$ into a (hollow) Wigner matrix plus a residual matrix and then showing that the residual matrix has a negligible effect on the overall spectrum.

First, adding and subtracting $F(A)$ in the definition of $\Gamma$ yields,

$$\Gamma = \{\widetilde{R} - F(A)\} + \{F(A) - 2^{-1}(J - I)\}. \tag{1}$$

For each $1 \leq i \leq N$, let $U_{(i)}$ denote the $i$-th order statistic of the sample $\{F(A_{kj})\}_{k<j}$. The difference between the $i$-th order statistic of $\{\widetilde{R}_{kj}\}_{k<j}$ and $\{U_{(i)}\}_{1\leq i\leq N}$ is thus $i/(N+1) - U_{(i)}$, hence expanding the squared Frobenius norm of $\widetilde{R} - F(A)$ yields

$$\|\widetilde{R} - F(A)\|_{\mathrm{F}}^2 = 2\sum_{k<j}\left\{\widetilde{R}_{kj} - F(A_{kj})\right\}^2 = 2\sum_{i=1}^{N}\left(\frac{i}{N+1} - U_{(i)}\right)^2.$$

It is well-known that the order statistics of a random sample from the standard uniform distribution are Beta distributed with $U_{(i)} \sim \mathrm{Beta}(i, N+1-i)$. Furthermore, from Marchal & Arbel (2017, Theorem 2.1), for each $1 \leq i \leq N$ the order statistic $U_{(i)}$ is a sub-Gaussian random variable with optimal proxy variance satisfying $\sigma_{\mathrm{opt}}^2 \leq 1/\{4(N+2)\}$, hence its moment generating function

satisfies

$$E\left(\exp\left[t\left\{U_{(i)}-\frac{i}{N+1}\right\}\right]\right)\le\exp\left(\frac{\sigma_{\mathrm{opt}}^2t^2}{2}\right)\le\left(\frac{t^2}{8(N+2)}\right).$$

By applying Vershynin (2018, Proposition 2.5.2) and the above bound, there exists a universal constant $C>0$ such that for all $1\le i\le N$ and any $t>0$,

$$\mathrm{pr}\left(\left|U_{(i)}-\frac{i}{N+1}\right|>t\right)\le\exp(-CNt^2).$$

Combining the above observations yields the tail probability bound

$$\begin{aligned}\mathrm{pr}\left(\|\widetilde{R}-F(A)\|_{\mathrm{F}}>\log n\right)&=\mathrm{pr}\left\{\sum_{i=1}^{N}\left(\frac{i}{N+1}-U_{(i)}\right)^2>\frac{(\log n)^2}{2}\right\}\\&\le\sum_{i=1}^{N}\mathrm{pr}\left\{\left(\frac{i}{N+1}-U_{(i)}\right)^2>\frac{(\log n)^2}{2N}\right\}\\&\le N\exp\left\{-\frac{C(\log n)^2}{2}\right\}\\&=Nn^{-2^{-1}C\log n}.\end{aligned}\tag{2}$$

Hence, by slight abuse of notation,

$$\sum_{n=1}^{\infty}\mathrm{pr}\left(n^{-1/2}\|\widetilde{R}-F(A)\|_{\mathrm{F}}>n^{-1/2}\log n\right)<\infty,$$

so by a direct application of the Borel–Cantelli lemma, it follows that

$$\limsup_{n\to\infty}n^{-1/2}\|\widetilde{R}-F(A)\|_{\mathrm{F}}=0\qquad\text{almost surely.}\tag{3}$$

Letting $F_n^{(1)}$ and $F_n^{(2)}$ denote the empirical spectral distributions of $n^{-1/2}\Gamma$ and $n^{-1/2}\{F(A)-2^{-1}(J-I)\}$ respectively, Lemma 1 and Eq. (3) ensure that $L(F_n^{(1)},F_n^{(2)})\to 0$ almost surely as $n\to\infty$. Since $\sigma_n^{-1}\{F(A)-2^{-1}(J-I)\}$ is a (hollow) standard Wigner matrix, the semicircle law holds for $\sigma_n^{-1}\{F(A)-2^{-1}(J-I)\}$. To reiterate, $\mu_n$ denotes the empirical spectral distribution of $n^{-1/2}W\equiv\sigma_n^{-1}n^{-1/2}\Gamma$, and $\mu$ denotes the semicircle distribution. Lemma 1 and Lemma 2 guarantee that for all $f\in C_b(\mathbb{R})$,

$$\lim_{n\to\infty}\int_{\mathbb{R}}f(x)\mu_n(\mathrm{d}x)=\int_{\mathbb{R}}f(x)\mu(\mathrm{d}x)\qquad\text{almost surely.}$$

This establishes the semicircle law for $n^{-1/2}W$.

Next, we prove the convergence of the spectral norm. From Eq. (1),

$$\|F(A)-2^{-1}(J-I)\|-\|\widetilde{R}-F(A)\|\le\|\Gamma\|\le\|F(A)-2^{-1}(J-I)\|+\|\widetilde{R}-F(A)\|.\tag{4}$$

The matrix $F(A)-2^{-1}(J-I)$ is symmetric with bounded and mean zero entries. Additionally, the entry variance is $\sigma^2\equiv 1/12=\sigma_n^2+O(n^{-2})$. According to Bai & Yin (1988, Theorem A),

$$\lim_{n\to\infty}\sigma^{-1}n^{-1/2}\left\|F(A)-2^{-1}(J-I)\right\|=2\qquad\text{almost surely,}$$

which in turn implies that

$$\lim_{n\to\infty} \sigma_n^{-1} n^{-1/2} \left\| F(A) - 2^{-1}(J - I) \right\| = 2 \qquad \text{almost surely.}$$

Thus, Eq. (4) together with Eq. (3) guarantees

$$\lim_{n\to\infty} n^{-1/2} \|W\| = \lim_{n\to\infty} \sigma_n^{-1} n^{-1/2} \|\Gamma\| = 2 \qquad \text{almost surely.}$$

This concludes the proof of Theorem 1. □

*Proof of Theorem 2.* This is a special case of Lemma 7. □

*Proof of Theorem 3.* Recall that $\widetilde{R} + 2^{-1}I = 2^{-1}J + \Gamma$. For ease of presentation, let $\widehat{\lambda}_1 \geq \cdots \geq \widehat{\lambda}_n$ denote the eigenvalues of $\widetilde{R} + 2^{-1}I$ in descending order, and let $\widehat{u}_1, \ldots, \widehat{u}_n$ denote corresponding orthonormal eigenvectors. Additionally, write $\lambda_1 \equiv \lambda_1(2^{-1}J) = n/2$ and $u_1 = n^{-1/2}1_n$. By direct computation,

$$(\widehat{\lambda}_1 I - \Gamma)\widehat{u}_1 = (\widetilde{R} + 2^{-1}I)\widehat{u}_1 - \Gamma\widehat{u}_1 = 2^{-1}J\widehat{u}_1 = \lambda_1 u_1 u_1^{\mathrm{T}} \widehat{u}_1. \tag{5}$$

To bound the difference of leading eigenvalues, an application of Weyl's inequality yields

$$|\widehat{\lambda}_1 - \lambda_1| \leq \|\Gamma\|. \tag{6}$$

Theorem 2 ensures that $\|\Gamma\| = O(n^{1/2})$ with high probability, hence necessarily $\widehat{\lambda}_1 = O(n)$ with high probability. Consequently, $\widehat{\lambda}_1 I - \Gamma$ is invertible with high probability. Left multiplying Eq. (5) by $u_1^{\mathrm{T}}(\widehat{\lambda}_1 I - \Gamma)^{-1}$ yields

$$u_1^{\mathrm{T}}\widehat{u}_1 = \lambda_1 u_1^{\mathrm{T}}(\widehat{\lambda}_1 I - \Gamma)^{-1} u_1 u_1^{\mathrm{T}} \widehat{u}_1. \tag{7}$$

Yu et al. (2015, Corollary 1) ensures that

$$\sin\Theta(u_1, \widehat{u}_1) \leq \frac{2\|\Gamma\|}{n/2} = O(n^{-1/2}) \tag{8}$$

with high probability. Since $0 \leq u_1^{\mathrm{T}}\widehat{u}_1 = \cos\Theta(u_1, \widehat{u}_1) = \{1 - \sin^2\Theta(u_1, \widehat{u}_1)\}^{1/2}$, it follows from Eq. (8) that $u_1^{\mathrm{T}}\widehat{u}_1$ is bounded away from zero with high probability. Dividing both sides of Eq. (7) by $u_1^{\mathrm{T}}\widehat{u}_1$ thus yields the identity

$$1 = \lambda_1 u_1^{\mathrm{T}}(\widehat{\lambda}_1 I - \Gamma)^{-1} u_1. \tag{9}$$

From Eq. (6) and Theorem 2, the quantity $\|\widehat{\lambda}_1^{-1}\Gamma\|$ is well-defined and satisfies $\|\widehat{\lambda}_1^{-1}\Gamma\| < 1$. Thus, Eq. (9) can be rewritten using the von Neumann matrix series expansion as

$$\begin{aligned} 1 &= \frac{\lambda_1}{\widehat{\lambda}_1} u_1^{\mathrm{T}} \left( I - \frac{\Gamma}{\widehat{\lambda}_1} \right)^{-1} u_1 \\ &= \frac{\lambda_1}{\widehat{\lambda}_1} u_1^{\mathrm{T}} \left( I + \sum_{l=1}^{\infty} \widehat{\lambda}_1^{-l} \Gamma^l \right) u_1 \\ &= \frac{\lambda_1}{\widehat{\lambda}_1} + \sum_{l=1}^{\infty} \frac{\lambda_1}{\widehat{\lambda}_1^{l+1}} u_1^{\mathrm{T}} \Gamma^l u_1. \end{aligned} \tag{10}$$

Applying $\widehat{\lambda}_1 = O_p(n)$ together with Theorem 2, there exists a fixed, smallest integer $L > 0$ such that the tail of the series satisfies the operator norm bound

$$\left\| \sum_{l=L+1}^{\infty} \widehat{\lambda}_1^{-(l+1)} \Gamma^l \right\| = O_p \left\{ n^{(L+1)/2} \widehat{\lambda}_1^{-(L+2)} \right\} = O_p(n^{-4}).$$

Thus, proceeding with the earlier calculation yields the approximation

$$1 = \frac{\lambda_1}{\widehat{\lambda}_1} + \sum_{l=1}^{L} \frac{\lambda_1}{\widehat{\lambda}_1^{l+1}} u_1^{\mathrm{T}} \Gamma^l u_1 + O_p(n^{-3}). \tag{11}$$

Multiplying through by $\widehat{\lambda}_1$ and then subtracting $\lambda_1$ yields

$$\widehat{\lambda}_1 - \lambda_1 = \sum_{l=1}^{L} \frac{\lambda_1}{\widehat{\lambda}_1^{l}} u_1^{\mathrm{T}} \Gamma^l u_1 + O_p(n^{-2}). \tag{12}$$

Now, observe that applying the bounds in Lemma 5 and Lemma 6 yields

$$u_1^{\mathrm{T}} \Gamma^l u_1 = u_1^{\mathrm{T}} \{ \Gamma^l - E(\Gamma^l) \} u_1 + u_1^{\mathrm{T}} E(\Gamma^l) u_1 = \begin{cases} O_p\{n^{l/2}\} & \text{when } l \text{ is even,} \\ O_p\{n^{(l-1)/2}\} & \text{when } l \text{ is odd.} \end{cases} \tag{13}$$

Thus, the above summation of $L$ terms admits the approximation

$$\sum_{l=1}^{L} \frac{\lambda_1}{\widehat{\lambda}_1^{l}} u_1^{\mathrm{T}} \Gamma^l u_1 = \frac{\lambda_1}{\widehat{\lambda}_1} u_1^{\mathrm{T}} \Gamma u_1 + \frac{\lambda_1}{\widehat{\lambda}_1^{2}} u_1^{\mathrm{T}} \Gamma^2 u_1 + O_p(n^{-1}). \tag{14}$$

Next, applying Eq. (13) to Eq. (11) yields

$$\lambda_1 / \widehat{\lambda}_1 = 1 + O_p(n^{-1}), \tag{15}$$

hence from Eq. (12) and Eq. (14), it follows that the eigenvalue difference satisfies

$$\widehat{\lambda}_1 - \lambda_1 = u_1^{\mathrm{T}} \Gamma u_1 + \frac{1}{\lambda_1} u_1^{\mathrm{T}} \Gamma^2 u_1 + O_p(n^{-1}). \tag{16}$$

Further, by direct computation, $u_1^{\mathrm{T}} \Gamma u_1 = 0$ holds almost surely. Eq. (16) therefore becomes

$$\widehat{\lambda}_1(\widetilde{R}) - \frac{n-1}{2} = \frac{u_1^{\mathrm{T}} \Gamma^2 u_1}{\lambda_1} + O_p(n^{-1}).$$

Finally, invoking Lemma 8 concludes the proof of Theorem 3. □

*Proof of Theorem 4.* See Füredi & Komlós (1981). □

*Proof of Theorem 5.* This proof proceeds by decomposing the bilinear form $u_1^{\mathrm{T}} \widehat{u}_1 \widehat{u}_1^{\mathrm{T}} u_1$ using Cauchy's residue theorem. Such an approach was previously used in Fan et al. (2022) but in the context of independent-entry noise models.

Recall that $\lambda_1 = n/2$. Let $c_0$ be a small real-valued constant satisfying $0 < c_0 < 1$. Define a contour $\Omega_1$ centered at $(a+b)/2$ with radius $|a-b|/2$, where $a = \lambda_1/(1+c_0)$ and $b = (1+c_0)\lambda_1$. From Weyl's inequality and Theorem 2, the difference of leading eigenvalues satisfies

$$|\widehat{\lambda}_1 - \lambda_1| \leq \|\widetilde{R} + 2^{-1} I - 2^{-1} J\| = \|\Gamma\| = O(n^{1/2})$$

with high probability. Since $\lambda_1 = n/2$, the above inequality ensures that $\Omega_1$ encloses $\widehat{\lambda}_1$ with high probability.

For $j = 2, \dots, n$, it follows from the triangle inequality that

$$|\widehat{\lambda}_j - \lambda_1| = |\widehat{\lambda}_j - \lambda_j + \lambda_j - \lambda_1| \geq |\lambda_j - \lambda_1| - |\widehat{\lambda}_j - \lambda_j|.$$

Weyl's inequality guarantees that $|\widehat{\lambda}_j - \lambda_j| \leq \|\Gamma\|$ for all $j$, hence $|\widehat{\lambda}_j - \lambda_1| \geq |\lambda_1| - \|\Gamma\|$ for $j = 2, \dots, n$. Thus, with high probability, $\Omega_1$ does not enclose $\widehat{\lambda}_j$ for $j = 2, \dots, n$. The definition of $\Omega_1$, together with Cauchy's residue theorem yields that

$$-\frac{1}{2\pi \mathrm{i}} \oint_{\Omega_1} \frac{1}{\widehat{\lambda}_1 - z} \mathrm{d}z = 1, \qquad \text{and} \qquad -\frac{1}{2\pi \mathrm{i}} \oint_{\Omega_1} \frac{1}{\widehat{\lambda}_j - z} \mathrm{d}z = 0, \quad j \geq 2,$$

both with high probability.

On the event that $\Omega_1$ encloses $\widehat{\lambda}_1$ and does not enclose $\widehat{\lambda}_j$ for $j = 2, \dots, n$, it holds that

$$\begin{aligned} u_1^{\mathrm{T}} \widehat{u}_1 \widehat{u}_1^{\mathrm{T}} u_1 &= -\frac{u_1^{\mathrm{T}} \widehat{u}_1 \widehat{u}_1^{\mathrm{T}} u_1}{2\pi \mathrm{i}} \oint_{\Omega_1} \frac{1}{\widehat{\lambda}_1 - z} \mathrm{d}z \\ &= -\frac{1}{2\pi \mathrm{i}} \oint_{\Omega_1} u_1^{\mathrm{T}} \left( \sum_{j=1}^{n} \frac{\widehat{u}_j \widehat{u}_j^{\mathrm{T}}}{\widehat{\lambda}_j - z} \right) u_1 \mathrm{d}z \\ &= -\frac{1}{2\pi \mathrm{i}} \oint_{\Omega_1} u_1^{\mathrm{T}} (\widetilde{R} + 2^{-1} I - zI)^{-1} u_1 \mathrm{d}z \\ &= -\frac{1}{2\pi \mathrm{i}} \oint_{\Omega_1} u_1^{\mathrm{T}} (\Gamma - zI + \lambda_1 u_1 u_1^{\mathrm{T}})^{-1} u_1 \mathrm{d}z. \end{aligned} \tag{17}$$

Next, by the Sherman–Morrison–Woodbury formula, for any invertible matrix $A$ and vectors $u$, $v$ with appropriate dimensions, if $v^{\mathrm{T}} A^{-1} u + 1 \neq 0$, then

$$(A + uv^{\mathrm{T}})^{-1} = A^{-1} - \frac{A^{-1} u v^{\mathrm{T}} A^{-1}}{1 + v^{\mathrm{T}} A^{-1} u}.$$

In particular, direct computation subsequently gives

$$v^{\mathrm{T}} (A + uv^{\mathrm{T}})^{-1} u = \frac{v^{\mathrm{T}} A^{-1} u}{1 + v^{\mathrm{T}} A^{-1} u}.$$

Thus, applying the Sherman–Morrison–Woodbury formula inside the integral in Eq. (17) yields

$$u_1^{\mathrm{T}} \widehat{u}_1 \widehat{u}_1^{\mathrm{T}} u_1 = -\frac{1}{2\pi \mathrm{i}} \oint_{\Omega_1} \frac{u_1^{\mathrm{T}} (\Gamma - zI)^{-1} u_1}{1 + \lambda_1 u_1^{\mathrm{T}} (\Gamma - zI)^{-1} u_1} \mathrm{d}z. \tag{18}$$

An intermediate step in Eq. (17) together with Eq. (18) shows that

$$u_1^{\mathrm{T}} \left( \sum_{j=1}^{n} \frac{\widehat{u}_j \widehat{u}_j^{\mathrm{T}}}{\widehat{\lambda}_j - z} \right) u_1 = \frac{u_1^{\mathrm{T}} (\Gamma - zI)^{-1} u_1}{1 + \lambda_1 u_1^{\mathrm{T}} (\Gamma - zI)^{-1} u_1}.$$

Now, using the definition of $\Omega_1$, with high probability $\widehat{\lambda}_1$ is the only singular point of $z \mapsto u_1^{\mathrm{T}} (\Gamma - zI)^{-1} u_1 / \{1 + \lambda_1 u_1^{\mathrm{T}} (\Gamma - zI)^{-1} u_1\}$ inside $\Omega_1$. By Cauchy's residue theorem, continuing

the calculation in Eq. (18) yields

$$u_1^{\mathrm{T}}\widehat{u}_1\widehat{u}_1^{\mathrm{T}}u_1 = -\lim_{z\to\widehat{\lambda}_1}\frac{(z-\widehat{\lambda}_1)u_1^{\mathrm{T}}(\Gamma-zI)^{-1}u_1}{1+\lambda_1 u_1^{\mathrm{T}}(\Gamma-zI)^{-1}u_1} = -\frac{\mathrm{d}\{(z-\widehat{\lambda}_1)u_1^{\mathrm{T}}(\Gamma-zI)^{-1}u_1\}/\mathrm{d}z\mid_{z=\widehat{\lambda}_1}}{\mathrm{d}\{1+\lambda_1 u_1^{\mathrm{T}}(\Gamma-zI)^{-1}u_1\}/\mathrm{d}z\mid_{z=\widehat{\lambda}_1}}. \tag{19}$$

Provided $\|\Gamma\|/|z| < 1$, expanding $(\Gamma - zI)^{-1}$ as a series representation yields

$$(\Gamma - zI)^{-1} = -\sum_{l=0}^{\infty}\frac{\Gamma^l}{z^{l+1}}. \tag{20}$$

Applying Eq. (20) to Eq. (19) gives

$$\begin{aligned} u_1^{\mathrm{T}}\widehat{u}_1\widehat{u}_1^{\mathrm{T}}u_1 &= \frac{\mathrm{d}\{(z-\widehat{\lambda}_1)\sum_{l=0}^{\infty} z^{-(l+1)}u_1^{\mathrm{T}}\Gamma^l u_1\}/\mathrm{d}z\mid_{z=\widehat{\lambda}_1}}{\mathrm{d}\{1-\lambda_1\sum_{l=0}^{\infty} z^{-(l+1)}u_1^{\mathrm{T}}\Gamma^l u_1\}/\mathrm{d}z\mid_{z=\widehat{\lambda}_1}} \\ &= \frac{\sum_{l=0}^{\infty}\widehat{\lambda}_1^{-(l+1)}u_1^{\mathrm{T}}\Gamma^l u_1}{\lambda_1(l+1)\sum_{l=0}^{\infty} z^{-(l+2)}u_1^{\mathrm{T}}\Gamma^l u_1} \\ &= \frac{\sum_{l=0}^{L}\widehat{\lambda}_1^{-(l+1)}u_1^{\mathrm{T}}\Gamma^l u_1 + O_p(n^{-4})}{\lambda_1\sum_{l=0}^{L}(l+1)\widehat{\lambda}_1^{-(l+2)}u_1^{\mathrm{T}}\Gamma^l u_1 + O_p(n^{-4})}, \end{aligned} \tag{21}$$

where $L > 0$ is the smallest integer that satisfies $\|\sum_{l=L+1}^{\infty}\widehat{\lambda}_1^{-(l+1)}\Gamma^l\| = O_p(n^{-4})$ as in the proof of Theorem 3.

Next, the objective is to further expand Eq. (21). To that end, dividing both sides of Eq. (16) by $\widehat{\lambda}_1$ yields

$$\frac{\lambda_1}{\widehat{\lambda}_1} = 1 - \frac{1}{\widehat{\lambda}_1}u_1^{\mathrm{T}}\Gamma u_1 - \frac{1}{\lambda_1\widehat{\lambda}_1}u_1^{\mathrm{T}}\Gamma^2 u_1 + O_p(n^{-2}). \tag{22}$$

Using Eq. (15) to approximate $\widehat{\lambda}_1$ with $\lambda_1$ in the right-hand side of Eq. (22) gives

$$\frac{\lambda_1}{\widehat{\lambda}_1} = 1 - \frac{1}{\lambda_1}u_1^{\mathrm{T}}\Gamma u_1 - \frac{1}{\lambda_1^2}u_1^{\mathrm{T}}\Gamma^2 u_1 + O_p(n^{-2}). \tag{23}$$

Now, Eq. (23) and Eq. (13) can be readily used to simplify Eq. (21), namely

$$\begin{aligned} u_1^{\mathrm{T}}\widehat{u}_1\widehat{u}_1^{\mathrm{T}}u_1 &= \frac{\sum_{l=0}^{L}\widehat{\lambda}_1^{-(l+1)}u_1^{\mathrm{T}}\Gamma^l u_1 + O_p(n^{-4})}{\lambda_1\sum_{l=0}^{L}(l+1)\widehat{\lambda}_1^{-(l+2)}u_1^{\mathrm{T}}\Gamma^l u_1 + O_p(n^{-4})} \\ &= \frac{u_1^{\mathrm{T}}u_1 + \widehat{\lambda}_1^{-1}u_1^{\mathrm{T}}\Gamma u_1 + \widehat{\lambda}_1^{-2}u_1^{\mathrm{T}}\Gamma^2 u_1 + O_p(n^{-2})}{\lambda_1(\widehat{\lambda}_1^{-1}u_1^{\mathrm{T}}u_1 + 2\widehat{\lambda}_1^{-2}u_1^{\mathrm{T}}\Gamma u_1 + 3\widehat{\lambda}_1^{-3}u_1^{\mathrm{T}}\Gamma^2 u_1) + O_p(n^{-2})} \\ &= \frac{1 + \lambda_1^{-1}u_1^{\mathrm{T}}\Gamma u_1 + \lambda_1^{-2}u_1^{\mathrm{T}}\Gamma^2 u_1 + O_p(n^{-2})}{\lambda_1/\widehat{\lambda}_1 + 2\lambda_1^{-1}u_1^{\mathrm{T}}\Gamma u_1 + 3\lambda_1^{-2}u_1^{\mathrm{T}}\Gamma^2 u_1 + O_p(n^{-2})} \\ &= \frac{1 + \lambda_1^{-1}u_1^{\mathrm{T}}\Gamma u_1 + \lambda_1^{-2}u_1^{\mathrm{T}}\Gamma^2 u_1 + O_p(n^{-2})}{1 + \lambda_1^{-1}u_1^{\mathrm{T}}\Gamma u_1 + 2\lambda_1^{-2}u_1^{\mathrm{T}}\Gamma^2 u_1 + O_p(n^{-2})} \\ &= 1 - \frac{1}{\lambda_1^2}u_1^{\mathrm{T}}\Gamma^2 u_1 + O_p(n^{-2}). \end{aligned} \tag{24}$$

Finally, taking square roots on both sides and applying a Taylor series expansion yields

$$u_1^{\mathrm{T}}\widehat{u}_1 = 1 - \frac{1}{2\lambda_1^2}u_1^{\mathrm{T}}\Gamma^2 u_1 + O_p(n^{-2}). \tag{25}$$

By applying Lemma 8, it follows that as $n \to \infty$,

$$n\widetilde{\sigma}_n^{-1}\left(u_1^{\mathrm{T}}\widehat{u}_1 - 1 + \frac{1}{6n}\right) \to N(0,1) \qquad \text{in distribution.}$$

This establishes the claim in Theorem 5 for $x^{\mathrm{T}}\widehat{u}_1$ under the special case $x = u_1$.

Next, this proof considers the linear form $x^{\mathrm{T}}\widehat{u}_1$ with a general unit vector $x$. First, by Eq. (5),

$$(\widehat{\lambda}_1 I - \Gamma)\widehat{u}_1 = \lambda_1 u_1 u_1^{\mathrm{T}}\widehat{u}_1.$$

Multiplying both sides by $x^{\mathrm{T}}(\widehat{\lambda}_1 I - \Gamma)^{-1}$ and plugging Eq. (25) and Eq. (23) into the resulting equation yields

$$\begin{aligned}
x^{\mathrm{T}}\widehat{u}_1 &= \lambda_1 x^{\mathrm{T}}(\widehat{\lambda}_1 I - \Gamma)^{-1}u_1\left(1 - \frac{1}{2\lambda_1^2}u_1^{\mathrm{T}}\Gamma^2 u_1\right) + O_p(n^{-2}) \\
&= \frac{\lambda_1}{\widehat{\lambda}_1}x^{\mathrm{T}}\left(I + \sum_{l=1}^{\infty}\widehat{\lambda}_1^{-l}\Gamma^l\right)u_1\left(1 - \frac{1}{2\lambda_1^2}u_1^{\mathrm{T}}\Gamma^2 u_1\right) + O_p(n^{-2}) \\
&= \frac{\lambda_1}{\widehat{\lambda}_1}x^{\mathrm{T}}u_1 + \frac{\lambda_1}{\widehat{\lambda}_1^2}x^{\mathrm{T}}\Gamma u_1 + \frac{\lambda_1}{\widehat{\lambda}_1^3}x^{\mathrm{T}}\Gamma^2 u_1 - \frac{1}{2\lambda_1^2}x^{\mathrm{T}}u_1 u_1^{\mathrm{T}}\Gamma^2 u_1 + O_p(n^{-2}) \\
&= \left(1 - \frac{3u_1^{\mathrm{T}}\Gamma^2 u_1}{2\lambda_1^2}\right)x^{\mathrm{T}}u_1 + \frac{x^{\mathrm{T}}\Gamma u_1}{\lambda_1} + \frac{x^{\mathrm{T}}\Gamma^2 u_1}{\lambda_1^2} + O_p(n^{-2}) \\
&= \left\{1 - \frac{3E(u_1^{\mathrm{T}}\Gamma^2 u_1)}{2\lambda_1^2}\right\}x^{\mathrm{T}}u_1 + \frac{x^{\mathrm{T}}\Gamma u_1}{\lambda_1} + \frac{E(x^{\mathrm{T}}\Gamma^2 u_1)}{\lambda_1^2} \\
&\quad + \left\{-\frac{3u_1^{\mathrm{T}}\Gamma^2 u_1}{2\lambda_1^2} + \frac{3E(u_1^{\mathrm{T}}\Gamma^2 u_1)}{2\lambda_1^2}\right\}x^{\mathrm{T}}u_1 + \left\{\frac{x^{\mathrm{T}}\Gamma^2 u_1}{\lambda_1^2} - \frac{E(x^{\mathrm{T}}\Gamma^2 u_1)}{\lambda_1^2}\right\} + O_p(n^{-2}).
\end{aligned}$$

Lemma 6 ensures that

$$\left\{\frac{3u_1^{\mathrm{T}}\Gamma^2 u_1}{2\lambda_1^2} - \frac{3E(u_1^{\mathrm{T}}\Gamma^2 u_1)}{2\lambda_1^2}\right\} = O_p(n^{-3/2}),$$

and

$$\left\{\frac{x^{\mathrm{T}}\Gamma^2 u_1}{\lambda_1^2} - \frac{E(x^{\mathrm{T}}\Gamma^2 u_1)}{\lambda_1^2}\right\} = O_p(n^{-3/2}).$$

Combining these observations yields the approximation

$$x^{\mathrm{T}}\widehat{u}_1 = \left\{1 - \frac{3E(u_1^{\mathrm{T}}\Gamma^2 u_1)}{2\lambda_1^2}\right\}x^{\mathrm{T}}u_1 + \frac{x^{\mathrm{T}}\Gamma u_1}{\lambda_1} + \frac{E(x^{\mathrm{T}}\Gamma^2 u_1)}{\lambda_1^2} + O_p(n^{-3/2}).$$

If $\mathrm{var}(x^{\mathrm{T}}\Gamma u_1/\lambda_1) \gg n^{-3}$, namely if $n \times \mathrm{var}(x^{\mathrm{T}}\Gamma u_1) \to \infty$, then

$$x^{\mathrm{T}}\widehat{u}_1 - \left\{1 - \frac{3E(u_1^{\mathrm{T}}\Gamma^2 u_1)}{2\lambda_1^2}\right\} x^{\mathrm{T}}u_1 - \frac{E(x^{\mathrm{T}}\Gamma^2 u_1)}{\lambda_1^2} = \frac{x^{\mathrm{T}}\Gamma u_1}{\lambda_1} + o_p\left[\left\{\mathrm{var}\left(\frac{x^{\mathrm{T}}\Gamma u_1}{\lambda_1}\right)\right\}^{1/2}\right].$$

From this representation, the leading order term $x^{\mathrm{T}}\Gamma u_1/\lambda_1$ controls the behavior of the quantity $x^{\mathrm{T}}\widehat{u}_1$. We now proceed to prove the asymptotic normality of $x^{\mathrm{T}}\Gamma u_1$ in order to establish the asymptotic normality of $x^{\mathrm{T}}\widehat{u}_1$.

To facilitate the discussion of the bilinear term $x^{\mathrm{T}}\Gamma u_1$ with general vector pairs, we use $w = (w_1, \dots, w_n)^{\mathrm{T}}$ and $v = (v_1, \dots, v_n)^{\mathrm{T}}$ to denote two arbitrary unit vectors. In the following proof, we establish some additional notation and employ Hájek (1968, Theorem 2.1) to prove the asymptotic normality of $w^{\mathrm{T}}\Gamma v$. In particular, let $S$ denote the sum

$$S = w^{\mathrm{T}}\Gamma v = \sum_{i=1}^{n}\sum_{j=1}^{n}\Gamma_{ij}w_i v_j = \sum_{i<j}(w_i v_j + w_j v_i)\Gamma_{ij}.$$

For positive integer pairs $(i, j)$, define

$$p(i, j) = (i-1)(2n-i)/2 + (j-i),$$

and observe that this is a one-to-one mapping from $\{(i, j) : 1 \le i < j \le n\}$ to $[\![N]\!]$. Hence, $S$ can be rewritten as

$$S = \sum_{i=1}^{N} c_i \dot{\Gamma}_i,$$

and reindexing the expressions lets us write

$$c_i \equiv w_s v_t + w_t v_s, \qquad \dot{\Gamma}_i \equiv \Gamma_{st}, \qquad i = p(s, t).$$

In order to closely follow the notation and approach in Hájek (1968), define

$$a_N(i) = i/(N+1), \qquad \bar{\varphi} = \int_0^1 x\,\mathrm{d}x = 1/2,$$

$$H(x) = F(x), \qquad \bar{c} = \sum_{s \ne t} w_s v_t / N.$$

By direct calculation, $c_i - \bar{c}$ can be written as

$$c_i - \bar{c} = w_s v_t + w_t v_s - \sum_{s=1}^{n}\sum_{t=1}^{n} w_s v_t/N + \sum_{s=1}^{n} w_s v_s/N. \tag{26}$$

According to Hájek (1968, Theorem 2.1), for arbitrary $\epsilon > 0$, if

$$\mathrm{var}(S) \ge \{2\delta^{-1} + (2\epsilon^{-1/2}\beta^{-1} + 1) \times 5^{1/2}\}^2 \max_i (c_i - \bar{c})^2, \tag{27}$$

where $\delta \equiv \delta_\epsilon > 0$ is chosen according to an application of the Lindeberg condition and $\beta \equiv \beta_\epsilon > 0$ is related to the standard normal distribution, then

$$\sup_{x \in \mathbb{R}} \left| \mathrm{pr}\left[\{S - E(S)\} < x\{\mathrm{var}(S)\}^{1/2}\right] - \Phi(x) \right| < \epsilon,$$

where $\Phi$ denotes the cumulative distribution function of $N(0,1)$. In words, $S \equiv w^{\mathrm{T}}\Gamma v$ is asymptotically normal after centering and scaling provided Eq. (27) holds. It remains to verify the above condition is satisfied for $(x, u_1)$.

Eq. (26) reveals that uniformly for all $i = 1, \ldots, N$, when $N$ is large,

$$|c_i - \bar{c}| \le 5\|w\|_\infty \|v\|_\infty,$$

thus Eq. (27) is satisfied provided

$$\mathrm{var}(w^{\mathrm{T}}\Gamma v)/(\|w\|_\infty^2 \|v\|_\infty^2) \to \infty.$$

Now, let $w = x$, $v = u_1 = n^{-1/2}1_n$, so $\|x\|_\infty^2 \|u_1\|_\infty^2 = O(n^{-1})$. Thus, if $n \times \mathrm{var}(x^{\mathrm{T}}\Gamma u_1) \to \infty$, then

$$\mathrm{var}(x^{\mathrm{T}}\Gamma u_1)/(\|x\|_\infty^2 \|u_1\|_\infty^2) \to \infty.$$

Hence, asymptotic normality is established for $x^{\mathrm{T}}\Gamma u_1$ when $n \times \mathrm{var}(x^{\mathrm{T}}\Gamma u_1) \to \infty$. Further, under this condition, as $n \to \infty$,

$$\frac{x^{\mathrm{T}}\widehat{u}_1 - \left\{1 - 3E(u_1^{\mathrm{T}}\Gamma^2 u_1)/(2\lambda_1^2)\right\}x^{\mathrm{T}}u_1 - E(x^{\mathrm{T}}\Gamma^2 u_1)/\lambda_1^2}{\left\{\mathrm{var}(x^{\mathrm{T}}\Gamma u_1/\lambda_1)\right\}^{1/2}} \to N(0,1) \qquad \text{in distribution.}$$

This concludes the proof of Theorem 5. □

*Proof of Corollary 1.* By direct computation,

$$\left\|\widehat{u}_1\widehat{u}_1^{\mathrm{T}} - u_1 u_1^{\mathrm{T}}\right\|_{\mathrm{F}}^2 = \mathrm{tr}\{(\widehat{u}_1\widehat{u}_1^{\mathrm{T}} - u_1 u_1^{\mathrm{T}})^2\} = 2 - 2(u_1^{\mathrm{T}}\widehat{u}_1)^2.$$

From Eq. (25), we have

$$\left\|\widehat{u}_1\widehat{u}_1^{\mathrm{T}} - u_1 u_1^{\mathrm{T}}\right\|_{\mathrm{F}}^2 = \frac{2}{\lambda_1^2} u_1^{\mathrm{T}}\Gamma^2 u_1 + O_p(n^{-2}).$$

Finally, applying Lemma 8 yields the stated asymptotic normality of $\|\widehat{u}_1\widehat{u}_1^{\mathrm{T}} - u_1 u_1^{\mathrm{T}}\|_{\mathrm{F}}^2$. □

*Proof of Eq. (8) in the main text.* Theorem 2 guarantees that $\|\Gamma\| = O(n^{1/2})$ with probability at least $1 - \exp(-Cn)$. To analyze the asymptotic behavior of the expectations of $\|\widehat{u}_{\widetilde{R}}\widehat{u}_{\widetilde{R}}^{\mathrm{T}} - u_1 u_1^{\mathrm{T}}\|_{\mathrm{F}}^2$ and $\|\widehat{u}_A\widehat{u}_A^{\mathrm{T}} - u_1 u_1^{\mathrm{T}}\|_{\mathrm{F}}^2$, we first work directly on the high-probability event $\|\Gamma\| = O(n^{1/2})$ (more precisely, on a sequence of such events indexed by $n$) and finally apply a crude but sufficient bound on the complement.

On the event $\|\Gamma\| = O(n^{1/2})$, Eq. (21) in the proof of Theorem 5 implies

$$u_1^{\mathrm{T}}\widehat{u}_{\widetilde{R}}\widehat{u}_{\widetilde{R}}^{\mathrm{T}}u_1 = \frac{\sum_{l=0}^{L} \widehat{\lambda}_1^{-(l+1)} u_1^{\mathrm{T}}\Gamma^l u_1 + O(n^{-4})}{\lambda_1 \sum_{l=0}^{L}(l+1)\widehat{\lambda}_1^{-(l+2)} u_1^{\mathrm{T}}\Gamma^l u_1 + O(n^{-4})}. \tag{28}$$

Further, on the same event, Eq. (10) gives

$$\frac{\lambda_1}{\widehat{\lambda}_1} = 1 - \frac{1}{\lambda_1^2}u_1^{\mathrm{T}}\Gamma^2 u_1 + O(n^{-3/2}). \tag{29}$$

Substituting Eq. (29) into Eq. (28) yields

$$\begin{aligned} u_1^{\mathrm{T}}\widehat{u}_{\widetilde{R}}\widehat{u}_{\widetilde{R}}^{\mathrm{T}}u_1 &= \frac{1 + \lambda_1^{-2}u_1^{\mathrm{T}}\Gamma^2 u_1 + O(n^{-3/2})}{1 + 2\lambda_1^{-2}u_1^{\mathrm{T}}\Gamma^2 u_1 + O(n^{-3/2})} \\ &= 1 - \frac{1}{\lambda_1^2}u_1^{\mathrm{T}}\Gamma^2 u_1 + O(n^{-3/2}). \end{aligned} \tag{30}$$

Note that the representation of the bilinear form $u_1^{\mathrm{T}} \widehat{u}_{\widetilde{R}} \widehat{u}_{\widetilde{R}}^{\mathrm{T}} u_1$ in Eq. (30) closely resembles that in Eq. (24), differing primarily in the control of the remainder term. This discrepancy arises because Eq. (30) is derived under the sole condition $\|\Gamma\| = O(n^{1/2})$, whereas Eq. (24) additionally leverages Lemma 5 and Lemma 6, enabling a stronger bound on the remainder at the expense of a weaker probability guarantee.

By following the calculations in the proof of Corollary 1 and combining Eq. (30), we have

$$\|\widehat{u}_{\widetilde{R}} \widehat{u}_{\widetilde{R}}^{\mathrm{T}} - u_1 u_1^{\mathrm{T}}\|_{\mathrm{F}}^2 = 2 - 2(u_1^{\mathrm{T}} \widehat{u}_{\widetilde{R}})^2 = \frac{2}{\lambda_1^2} u_1^{\mathrm{T}} \Gamma^2 u_1 + O(n^{-3/2}).$$

Direct computation yields that

$$\frac{1}{\lambda_1^2} E(u_1^{\mathrm{T}} \Gamma^2 u_1) = \frac{1}{n\lambda_1^2} \sum_{i \neq j} E(\Gamma_{ij}^2) + \frac{1}{n\lambda_1^2} \sum_{j, i \neq k} E(\Gamma_{ij}\Gamma_{jk}) = \frac{1}{3(n-1)} + O(n^{-2}),$$

where the last equality follows from Proposition 1 in the main text. Consequently,

$$E\left(\|\widehat{u}_{\widetilde{R}} \widehat{u}_{\widetilde{R}}^{\mathrm{T}} - u_1 u_1^{\mathrm{T}}\|_{\mathrm{F}}^2\right) = \frac{2}{3(n-1)} + O(n^{-3/2}).$$

On the complement of the event $\|\Gamma\| = O(n^{1/2})$ which has probability not exceeding $\exp(-Cn)$, the Frobenius norm $\|\widehat{u}_{\widetilde{R}} \widehat{u}_{\widetilde{R}}^{\mathrm{T}} - u_1 u_1^{\mathrm{T}}\|_{\mathrm{F}}^2$ is trivially upper bounded by 2. Taking both the high-probability event and its complement into account, we obtain

$$E\left(\|\widehat{u}_{\widetilde{R}} \widehat{u}_{\widetilde{R}}^{\mathrm{T}} - u_1 u_1^{\mathrm{T}}\|_{\mathrm{F}}^2\right) = \frac{2}{3(n-1)} + O(n^{-3/2}).$$

Now, let $A$ be a hollow symmetric random matrix with i.i.d strictly upper triangular entries from $N(\mu, \sigma^2)$ with $\mu \neq 0$. Let $\widehat{u}_A$ denote the leading eigenvector of $A$, let $\lambda_A$ denote the leading eigenvalue of $E(A)$, and let $\Gamma_A = A - E(A)$. By, for example Chen et al. (2021, Eq. (3.12)), with probability exceeding $1 - O(n^{-8})$, we have $\|\Gamma_A\| \leq 5\sigma\sqrt{n}$. Analogous to the preceding discussion for $\widetilde{R}$, we proceed to control the expectation of $\|\widehat{u}_A \widehat{u}_A^{\mathrm{T}} - u_1 u_1^{\mathrm{T}}\|_{\mathrm{F}}^2$ on the high-probability event $\|\Gamma_A\| = O(n^{1/2})$ where $\sigma^2 = O(1)$, and we apply a crude but sufficient bound of 2 on the complement.

When $\|\Gamma_A\| = O(n^{1/2})$, Fan et al. (2022, Eq. (19)) and its corresponding proof in Fan et al. (2022, Supplementary Material A.5), provide a decomposition of the bilinear form $u_1^{\mathrm{T}} \widehat{u}_A \widehat{u}_A^{\mathrm{T}} u_1$ analogous to that of $\widehat{u}_{\widetilde{R}}$, given by

$$u_1^{\mathrm{T}} \widehat{u}_A \widehat{u}_A^{\mathrm{T}} u_1 = 1 - \frac{1}{\lambda_1^2} u_1^{\mathrm{T}} \Gamma_A^2 u_1 + O(n^{-3/2}). \tag{31}$$

Note that this decomposition might appear to imply Eq. (6) in the main text. However, the bound for the remainder in Eq. (31) is in fact less precise than that of Eq. (6), as it relies solely on $\|\Gamma_A\| = O(n^{1/2})$ without making any additional assumptions. In contrast, deriving Eq. (6) in the main text requires a more nuanced argument to control the remainder term with finer granularity, which is essential for establishing Eq. (7) in the main text.

Proceeding with the computation, it follows from Eq. (31) that

$$\|\widehat{u}_A \widehat{u}_A^{\mathrm{T}} - u_1 u_1^{\mathrm{T}}\|_{\mathrm{F}}^2 = \frac{2}{\lambda_A^2} u_1^{\mathrm{T}} \Gamma_A^2 u_1 + O(n^{-3/2}).$$

Evaluating the expectation of the first term yields

$$\frac{2}{\lambda_A^2} E(u_1^{\mathrm{T}} \Gamma_A^2 u_1) = \frac{2}{n\lambda_A^2} \sum_{i \neq j} E\{(\Gamma_A)_{ij}^2\} = \frac{2\sigma^2}{\mu^2(n-1)}.$$

Incorporating the crude bound of 2 on the complement yields

$$E(\|\widehat{u}_A \widehat{u}_A^{\mathrm{T}} - u_1 u_1^{\mathrm{T}}\|_{\mathrm{F}}^2) = O(n^{-8}) + \frac{2\sigma^2}{\mu^2(n-1)} + O(n^{-3/2}) = \frac{2\sigma^2}{\mu^2(n-1)} + O(n^{-3/2}).$$

Therefore, as $n \to \infty$,

$$\frac{E(\|\widehat{u}_{\widetilde{R}} \widehat{u}_{\widetilde{R}}^{\mathrm{T}} - u_1 u_1^{\mathrm{T}}\|_{\mathrm{F}}^2)}{E(\|\widehat{u}_A \widehat{u}_A^{\mathrm{T}} - u_1 u_1^{\mathrm{T}}\|_{\mathrm{F}}^2)} = \frac{2/\{3(n-1)\} + O(n^{-3/2})}{2\sigma^2/\{\mu^2(n-1)\} + O(n^{-3/2})} \to \frac{\mu^2}{3\sigma^2}.$$

This establishes Eq. (8) in the main text. □

*Comment on the proofs of the main theorems*

A byproduct of the bilinear representation in the proof of Theorem 5 is that with high probability,

$$u_1^{\mathrm{T}}(\widetilde{R} - \widehat{\lambda}_1 \widehat{u}_1 \widehat{u}_1^{\mathrm{T}}) u_1 = O(n^{-1}). \tag{32}$$

In contrast, a direct application of the Davis–Kahan theorem (Yu et al., 2015) only gives that with high probability,

$$u_1^{\mathrm{T}}(\widetilde{R} - \widehat{\lambda}_1 \widehat{u}_1 \widehat{u}_1^{\mathrm{T}}) u_1 = \sum_{j \neq 1}^{n} \widehat{\lambda}_j u_1^{\mathrm{T}} \widehat{u}_j \widehat{u}_j^{\mathrm{T}} u_1 = O(n^{-1/2}),$$

since with high probability $|\widehat{\lambda}_j| = O(n^{1/2})$ and $|u_1^{\mathrm{T}} \widehat{u}_j| = O(n^{-1})$ for all $j \geq 2$. Although the bound from applying the Davis–Kahan theorem holds with a stronger probability statement, the bound itself is much looser.

*Proof of Eq.* (32). From the definitions of $\widehat{\lambda}_1$, $\lambda_1$, and $\widehat{u}_1$, $u_1$, it follows that

$$u_1^{\mathrm{T}} \left( \sum_{j=1}^{n} \widehat{\lambda}_j \widehat{u}_j \widehat{u}_j^{\mathrm{T}} \right) u_1 = u_1^{\mathrm{T}} \left( \lambda_1 u_1 u_1^{\mathrm{T}} + \Gamma \right) u_1.$$

Rewriting the above equation yields

$$u_1^{\mathrm{T}} \widehat{u}_1 \widehat{u}_1^{\mathrm{T}} u_1 = \widehat{\lambda}_1^{-1} u_1^{\mathrm{T}} \left( \lambda_1 u_1 u_1^{\mathrm{T}} + \Gamma - \sum_{j=2}^{n} \widehat{\lambda}_j \widehat{u}_j \widehat{u}_j^{\mathrm{T}} \right) u_1.$$

Expanding the above equation further yields a decomposition of the bilinear form, namely

$$\begin{aligned} u_1^{\mathrm{T}} \widehat{u}_1 \widehat{u}_1^{\mathrm{T}} u_1 &= \frac{\lambda_1}{\widehat{\lambda}_1} + \frac{u_1^{\mathrm{T}} \Gamma u_1}{\widehat{\lambda}_1} - \sum_{j=2}^{n} \frac{\widehat{\lambda}_j}{\widehat{\lambda}_1} u_1^{\mathrm{T}} \widehat{u}_j \widehat{u}_j^{\mathrm{T}} u_1 \\ &= 1 - \frac{1}{\lambda_1^2} u_1^{\mathrm{T}} \Gamma^2 u_1 - \sum_{j \neq 1}^{n} \frac{\widehat{\lambda}_j}{\widehat{\lambda}_1} u_1^{\mathrm{T}} \widehat{u}_j \widehat{u}_j^{\mathrm{T}} u_1 + O_p(n^{-2}), \end{aligned}$$

where the second equality leverages Eq. (23). In contrast, Eq. (24) shows that

$$u_1^{\mathrm{T}} \widehat{u}_1 \widehat{u}_1^{\mathrm{T}} u_1 = 1 - \frac{1}{\lambda_1^2} u_1^{\mathrm{T}} \Gamma^2 u_1 + O_p(n^{-2}).$$

Eq. (32) follows by comparing the two decompositions of $u_1^{\mathrm{T}}\widehat{u}_1\widehat{u}_1^{\mathrm{T}}u_1$ above, together with the fact that $\widehat{\lambda}_1 = O_p(n)$. □

## PROOFS FOR HYPOTHESIS TESTING APPLICATIONS

### *Setup: graph theory terminology*

The proofs below involve extensive discussion of graph enumeration. We begin by defining key terminology here to facilitate readability.

A *multigraph* $G = (V, E)$ is an ordered pair consisting of a finite set of vertices (nodes) $V$ connected by edges (links) in the multiset $E$. Throughout the proofs that follow, all graphs are undirected, meaning that all edges are bidirectional.

Two edges $\{i, j\}$ and $\{I, J\}$ are said to have *common nodes* if at least one of the following conditions holds: $i = I$ or $i = J$, or $j = I$ or $j = J$. In contrast, an edge $\{i, j\}$ is called an *isolated edge* if it does not have common nodes with any other edges.

If two edges $\{i, j\}$ and $\{I, J\}$ are not identical, then they are said to be *distinct*. An edge is called a *single edge* if it is distinct from all other edges in the graph. A multigraph $G = (V, E)$ has $d$ distinct edges if the *underlying set* of $E$ has cardinality $d$. For example, for a multigraph $G = (V, E)$, if $E = \{\{i_1, i_2\}, \{i_3, i_4\}, \{i_2, i_1\}\}$, then there are 2 distinct edges in $G$, namely $\{i_1, i_2\}$ and $\{i_3, i_4\}$. An edge is called a *repeated edge* if it is not a single edge.

A *chain* is an alternating sequence of nodes and edges, beginning and ending with nodes, in which each edge is incident with the two nodes immediately preceding and following it. Additionally, *length* describes the number of edges in a chain. For example, $\{a, b\}$ and $\{b, c\}$ together form a chain of length two.

Two multigraphs $G_1 = (V_1, E_1)$ and $G_2 = (V_2, E_2)$ are said to be *isomorphic* if there exists a pair of bijections $\alpha : V_1 \longrightarrow V_2$, $\beta : E_1 \longrightarrow E_2$ such that for all $e \in E_1$, the endpoints of $\beta(e)$ are the images under $\alpha$ of the endpoints of $e$. Otherwise, two graphs are said to be *non-isomorphic*. Formally, graph isomorphism is an equivalence relation on the space of graphs.

### *Setup: preliminaries for perturbation analysis*

Under the alternative hypotheses in both Setting 1 (community detection) and Setting 2 (principal submatrix detection), the data matrix $A$ can be viewed as generated from a weighted stochastic blockmodel (SBM) as follow, adopting the same notation as in Cape et al. (2024).

Let $\mathcal{F} \equiv \mathcal{F}^K = \{F_{(k,k')} : 1 \le k \le k' \le K\}$ denote a collection of $K(K+1)/2$ absolutely continuous cumulative distribution functions and define $F_{(k,k')} = F_{(k',k)}$ when $k > k'$. Let $g : [\![n]\!] \longrightarrow [\![K]\!]$ be the membership mapping function assigning each node $i \in [\![n]\!]$ to its block membership $g(i) \equiv g_i \in [\![K]\!]$. Then, $A$ has the form of a symmetric data matrix with latent blockmodel structure, namely,

$$A_{ij} = \begin{cases} \text{independent } F_{(g_i, g_j)} & \text{if } i \le j, \\ A_{ji} & \text{if } i > j. \end{cases}$$

Let $\Theta \in \{0, 1\}^{n \times K}$ be the so-called membership matrix where $\Theta_{ig_i} = 1$ for $i = 1, \ldots, n$ and all remaining entries are equal to zero. Let $\widetilde{R}$ be the matrix of normalized rank statistics derived from $A$. Let $\widetilde{B} \in [0, 1]^{K \times K}$ denote the symmetric matrix of expected normalized rank statistics, where

$$E(\widetilde{R}_{ij}) = \begin{cases} \widetilde{B}_{g_i, g_j} & \text{if } i \ne j, \\ 0 & \text{if } i = j. \end{cases}$$

As before, write $\Gamma = \widetilde{R} - E(\widetilde{R})$. We have

$$\widetilde{R} + \mathrm{diag}(\Theta\widetilde{B}\Theta^{\mathrm{T}}) = \Theta\widetilde{B}\Theta^{\mathrm{T}} + \Gamma.$$

Let $\widehat{\lambda}_1 \geq \ldots \geq \widehat{\lambda}_n$ denote the eigenvalues of the matrix $\widetilde{R} + \mathrm{diag}(\Theta\widetilde{B}\Theta^{\mathrm{T}})$, and let $\widehat{u}_1, \ldots, \widehat{u}_n$ denote corresponding orthonormal eigenvectors. Under all alternative hypotheses in this paper, $\widetilde{B}$ is full rank, hence $\Theta\widetilde{B}\Theta^{\mathrm{T}}$ has $K$ non-zero eigenvalues. Let $\lambda_1 \geq \ldots \geq \lambda_K$ denote the non-zero eigenvalues of $\Theta\widetilde{B}\Theta^{\mathrm{T}}$ with corresponding orthonormal eigenvectors $u_1, \ldots, u_K$.

Using the above definitions, direct computation yields

$$(\widehat{\lambda}_1 I - \Gamma)\widehat{u}_1 = \{\widetilde{R} + \mathrm{diag}(\Theta\widetilde{B}\Theta^{\mathrm{T}}) - \Gamma\}\widehat{u}_1 = (\Theta\widetilde{B}\Theta^{\mathrm{T}})\widehat{u}_1 = \left(\sum_{j=1}^{K} \lambda_j u_j u_j^{\mathrm{T}}\right)\widehat{u}_1.$$

Weyl's inequality yields $|\widehat{\lambda}_1 - \lambda_1| \leq \|\Gamma\|$, while Lemma 7 ensures that $\|\Gamma\| = O(n^{1/2})$ with high probability. Hence, in both Setting 1 and Setting 2, $\widehat{\lambda}_1 I - \Gamma$ is invertible and $\|\widehat{\lambda}_1^{-1}\Gamma\| < 1$ with high probability from the fact that $K = 2$ and $\lambda_1 = O(n)$. Therefore, by applying the preceding display equation, we obtain the perturbation expansion

$$\begin{aligned}
u_1^{\mathrm{T}}\widehat{u}_1 &= u_1^{\mathrm{T}}(\widehat{\lambda}_1 I - \Gamma)^{-1}\left(\sum_{j=1}^{K} \lambda_j u_j u_j^{\mathrm{T}}\right)\widehat{u}_1 \\
&= \sum_{j=1}^{K} \frac{\lambda_j}{\widehat{\lambda}_1} u_1^{\mathrm{T}} \left(I - \frac{\Gamma}{\widehat{\lambda}_1}\right)^{-1} u_j u_j^{\mathrm{T}}\widehat{u}_1 \\
&= \frac{\lambda_1}{\widehat{\lambda}_1} u_1^{\mathrm{T}} \left(I - \frac{\Gamma}{\widehat{\lambda}_1}\right)^{-1} u_1 u_1^{\mathrm{T}}\widehat{u}_1 + \sum_{j\neq 1}^{K} \frac{\lambda_j}{\widehat{\lambda}_1} u_1^{\mathrm{T}} \left(I - \frac{\Gamma}{\widehat{\lambda}_1}\right)^{-1} u_j u_j^{\mathrm{T}}\widehat{u}_1 \\
&= \frac{\lambda_1}{\widehat{\lambda}_1} u_1^{\mathrm{T}} \left(I + \sum_{l=1}^{\infty} \widehat{\lambda}_1^{-l}\Gamma^l\right) u_1 u_1^{\mathrm{T}}\widehat{u}_1 + \sum_{j\neq 1}^{K} \frac{\lambda_j}{\widehat{\lambda}_1} u_1^{\mathrm{T}} \left(I + \sum_{l=1}^{\infty} \widehat{\lambda}_1^{-l}\Gamma^l\right) u_j u_j^{\mathrm{T}}\widehat{u}_1.
\end{aligned}$$

As in the proof of Theorem 3, the Davis–Kahan theorem guarantees that $u_1^{\mathrm{T}}\widehat{u}_1$ is bounded away from zero with high probability. Dividing both sides of the above equation by $u_1^{\mathrm{T}}\widehat{u}_1$ therefore yields the identity

$$1 = \frac{\lambda_1}{\widehat{\lambda}_1} + \sum_{l=1}^{\infty} \frac{\lambda_1}{\widehat{\lambda}_1^{l+1}} u_1^{\mathrm{T}}\Gamma^l u_1 + \sum_{j\neq 1}^{K} \sum_{l=1}^{\infty} \frac{\lambda_j}{\widehat{\lambda}_1^{l+1}} u_1^{\mathrm{T}}\Gamma^l u_j \frac{u_j^{\mathrm{T}}\widehat{u}_1}{u_1^{\mathrm{T}}\widehat{u}_1},$$

hence the difference between the leading eigenvalues has the form

$$\widehat{\lambda}_1 - \lambda_1 = \sum_{l=1}^{\infty} \frac{\lambda_1}{\widehat{\lambda}_1^{l}} u_1^{\mathrm{T}}\Gamma^l u_1 + \sum_{j\neq 1}^{K} \sum_{l=1}^{\infty} \frac{\lambda_j}{\widehat{\lambda}_1^{l}} u_1^{\mathrm{T}}\Gamma^l u_j \frac{u_j^{\mathrm{T}}\widehat{u}_1}{u_1^{\mathrm{T}}\widehat{u}_1}.$$

Similar to the proof of Theorem 3, let $L > 0$ denote the smallest integer satisfying

$$\left\| \sum_{l=L+1}^{\infty} \widehat{\lambda}_1^{-(l+1)}\Gamma^l \right\| = O_p\left\{n^{(L+1)/2}\widehat{\lambda}_1^{-(L+2)}\right\} = O_p(n^{-4}),$$

hence

$$\widehat{\lambda}_1 - \lambda_1 = \sum_{l=1}^{L} \frac{\lambda_1}{\widehat{\lambda}_1^l} u_1^{\mathrm{T}} \Gamma^l u_1 + \sum_{j \neq 1}^{K} \sum_{l=1}^{L} \frac{\lambda_j}{\widehat{\lambda}_1^l} u_1^{\mathrm{T}} \Gamma^l u_j \frac{u_j^{\mathrm{T}} \widehat{u}_1}{u_1^{\mathrm{T}} \widehat{u}_1} + O_p(n^{-2}). \tag{33}$$

By Yu et al. (2015, Corollary 3), there exists a constant $C > 0$, such that

$$1 - u_1^{\mathrm{T}} \widehat{u}_1 = \frac{1}{2} \|u_1 - \widehat{u}_1\|^2 \leq \frac{C^2 \|\Gamma\|^2}{|\lambda_1 - \lambda_2|^2}. \tag{34}$$

In both Setting 1 and Setting 2, $|\lambda_1 - \lambda_2| = O(n)$ holds. Applying Lemma 7 to Eq. (34) therefore yields

$$1 - u_1^{\mathrm{T}} \widehat{u}_1 = O(n^{-1}) \tag{35}$$

with high probability. On the other hand, for $1 < j \leq K$, it holds that

$$\begin{aligned} |u_j^{\mathrm{T}} \widehat{u}_1| &= \frac{|u_j^{\mathrm{T}} (\lambda_j - \widehat{\lambda}_1) \widehat{u}_1|}{|\lambda_j - \widehat{\lambda}_1|} \\ &= \frac{|u_j^{\mathrm{T}} \{\Theta \widetilde{B} \Theta^{\mathrm{T}} - \widetilde{R} - \mathrm{diag}(\Theta \widetilde{B} \Theta^{\mathrm{T}})\} \widehat{u}_1|}{|\lambda_j - \widehat{\lambda}_1|} \\ &= \frac{|u_j^{\mathrm{T}} \Gamma \widehat{u}_1|}{|\lambda_j - \widehat{\lambda}_1|} \\ &\leq \frac{|u_j^{\mathrm{T}} \Gamma u_1 u_1^{\mathrm{T}} \widehat{u}_1|}{|\lambda_j - \widehat{\lambda}_1|} + \frac{|u_j^{\mathrm{T}} \Gamma (I - u_1 u_1^{\mathrm{T}}) \widehat{u}_1|}{|\lambda_j - \widehat{\lambda}_1|}. \end{aligned} \tag{36}$$

Now, Lemma 5 and Lemma 6 ensure that $|u_j^{\mathrm{T}} \Gamma u_1| = O_p(1)$ for all $j$, while applying the Davis–Kahan theorem per Yu et al. (2015) yields

$$\left\|(I - u_1 u_1^{\mathrm{T}}) \widehat{u}_1\right\| = \|\sin \Theta(u_1, \widehat{u}_1)\| \leq \frac{2\|\Gamma\|}{|\lambda_2 - \lambda_1|} = O_p(n^{-1/2}).$$

Applying the triangle inequality and Weyl's inequality yields

$$|\lambda_j - \widehat{\lambda}_1| \geq |\lambda_j - \lambda_1| - |\lambda_1 - \widehat{\lambda}_1| \geq |\lambda_j - \lambda_1| - \|\Gamma\| = O_p(n).$$

Applying these inequalities to Eq. (36) gives the overall bound

$$|u_j^{\mathrm{T}} \widehat{u}_1| \leq \frac{|u_j^{\mathrm{T}} \Gamma u_1| |u_1^{\mathrm{T}} \widehat{u}_1|}{|\lambda_j - \widehat{\lambda}_1|} + \frac{\|\Gamma\| \|(I - u_1 u_1^{\mathrm{T}}) \widehat{u}_1\|}{|\lambda_j - \widehat{\lambda}_1|} = O_p(n^{-1}). \tag{37}$$

Simplifying Eq. (33), Eq. (35), Eq. (37), together with Lemma 5 and Lemma 6, thus gives

$$\sum_{j \neq 1}^{K} \sum_{l=1}^{L} \frac{\lambda_j}{\widehat{\lambda}_1^l} u_1^{\mathrm{T}} \Gamma^l u_j \frac{u_j^{\mathrm{T}} \widehat{u}_1}{u_1^{\mathrm{T}} \widehat{u}_1} = O_p(n^{-1}). \tag{38}$$

Next, applying Lemma 5 and Lemma 6 gives

$$\sum_{l=1}^{L} \frac{\lambda_1}{\widehat{\lambda}_1} u_1^{\mathrm{T}} \Gamma^l u_1 = \frac{\lambda_1}{\widehat{\lambda}_1} u_1^{\mathrm{T}} \Gamma u_1 + \frac{\lambda_1}{\widehat{\lambda}_1^2} u_1^{\mathrm{T}} \Gamma^2 u_1 + O_p(n^{-1}). \tag{39}$$

Thus, plugging Eq. (38) and Eq. (39) into Eq. (33) yields

$$\widehat{\lambda}_1 - \lambda_1 = \frac{\lambda_1}{\widehat{\lambda}_1} u_1^{\mathrm{T}} \Gamma u_1 + \frac{\lambda_1}{\widehat{\lambda}_1^2} u_1^{\mathrm{T}} \Gamma^2 u_1 + O_p(n^{-1}). \tag{40}$$

Now, by dividing both sides by $\widehat{\lambda}_1$ and applying Lemma 5 and Lemma 6 again, it follows that

$$\lambda_1 / \widehat{\lambda}_1 = 1 + O_p(n^{-1}).$$

Finally, applying the above equation to Eq. (40) gives that under both Setting 1 and Setting 2,

$$\widehat{\lambda}_1 - \lambda_1 = u_1^{\mathrm{T}} \Gamma u_1 + \frac{1}{\lambda_1} u_1^{\mathrm{T}} \Gamma^2 u_1 + O_p(n^{-1}). \tag{41}$$

The remainder of this section is devoted to proving Proposition 2 and Proposition 3 in the main text. The proofs build upon the key decomposition given by Eq. (41).

*Proof of Proposition 2.* We begin this proof with several clarifying remarks. First, we shall make crucial use of Eq. (41) which establishes a decomposition for the leading eigenvalue in the general so-called $K$-block setting. Second, the asymptotic normality of the test statistic under the null hypothesis follows directly from Theorem 3. However, as noted in Section 3.2, when $E_1F_2 = 1/2$ holds, i.e., a situation that includes but is not identical to the null hypothesis, then the limiting behavior still holds. In the proof, we separately establish the stated asymptotic normality for this case.

Recall from the main text that $E_1F_2 = \int_{\mathbb{R}} F_2(x)\mathrm{d}F_1(x)$, and define $E_2F_1$ analogously. Similarly, write $E_1F_1F_2 = \int_{\mathbb{R}} F_1(x)F_2(x)\mathrm{d}F_1(x)$, and define $E_2F_1F_2$ analogously. Now, under the setting described in Eq. (10) of the main text, define $a = E(\widetilde{R}_{ij})$, $\sigma_a^2 = \mathrm{var}(\widetilde{R}_{ij})$, for $(i,j)$ satisfying $\theta_i\theta_j = 1$. Similarly, define $b = E(\widetilde{R}_{ij})$, $\sigma_b^2 = \mathrm{var}(\widetilde{R}_{ij})$, for $(i,j)$ satisfying $\theta_i\theta_j = -1$. Directly evaluating these expressions gives

$$\begin{aligned}
a &= \frac{1}{N+1}\left\{\frac{n}{4}\left(\frac{n}{2}-1\right) + \left(\frac{n}{2}\right)^2 \times E_1F_2 + \frac{1}{2}\right\},\\
b &= \frac{1}{N+1}\left\{\frac{n}{2}\left(\frac{n}{2}-1\right) \times E_2F_1 + \frac{1}{2}\left(\frac{n}{2}\right)^2 + \frac{1}{2}\right\},\\
\sigma_a^2 &= \frac{1}{48} + \frac{1}{4}E_1F_2^2 - \frac{1}{4}(E_1F_2)^2 + \frac{1}{2}E_1F_1F_2 - \frac{1}{4}E_1F_2 + O(n^{-1}),\\
\sigma_b^2 &= \frac{1}{48} + \frac{1}{4}E_2F_1^2 - \frac{1}{4}(E_2F_1)^2 + \frac{1}{2}E_2F_1F_2 - \frac{1}{4}E_2F_1 + O(n^{-1}).
\end{aligned} \tag{42}$$

Additionally, in what follows, it shall be convenient to make use of the identities

$$\begin{aligned}
E_1F_2 + E_2F_1 &= 1,\\
E_1F_2^2 &= 1 - 2E_2F_1F_2,\\
E_2F_1^2 &= 1 - 2E_1F_1F_2.
\end{aligned} \tag{43}$$

We now proceed with the remainder of the proof. Under the setting of Eq. (10) in the main text, it holds that $u_1 = n^{-1/2}1_n$. As mentioned previously, direct computation yields $u_1^{\mathrm{T}}\Gamma u_1 = 0$. Therefore, Eq. (41) becomes

$$\widehat{\lambda}_1 - \lambda_1 = \frac{1}{\lambda_1} u_1^{\mathrm{T}} \Gamma^2 u_1 + O_p(n^{-1}). \tag{44}$$

From the definitions of $\widehat{\lambda}_1$ and $\widehat{\lambda}_1(\widetilde{R})$, it holds that

$$\widehat{\lambda}_1(\widetilde{R}) = \widehat{\lambda}_1 - a. \tag{45}$$

By combining the fact that $\lambda_1 = (a+b)n/2$ with Eq. (42), Eq. (43), and Eq. (45), rewriting Eq. (44) in terms of $\widehat{\lambda}_1(\widetilde{R})$ yields

$$\widehat{\lambda}_1(\widetilde{R}) - \frac{1}{2}(n-1) = \frac{1}{\lambda_1} u_1^{\mathrm{T}} \Gamma^2 u_1 + O_p(n^{-1}).$$

Next, the leading order term decomposes in the manner

$$\frac{1}{\lambda_1} u_1^{\mathrm{T}} \Gamma^2 u_1 = \frac{1}{n\lambda_1} \sum_{k,i\neq j} \Gamma_{ki}\Gamma_{kj} + \frac{1}{n\lambda_1} \sum_{\theta_i\theta_j=1, i\neq j} \Gamma_{ij}^2 + \frac{1}{n\lambda_1} \sum_{\theta_i\theta_j=-1} \Gamma_{ij}^2.$$

To facilitate computation, define

$$M_n = \frac{1}{n\lambda_1} \sum_{k,i\neq j} \Gamma_{ki}\Gamma_{kj},$$

and define

$$\epsilon_n = \frac{1}{n\lambda_1} \sum_{\theta_i\theta_j=1, i\neq j} \Gamma_{ij}^2 + \frac{1}{n\lambda_1} \sum_{\theta_i\theta_j=-1} \Gamma_{ij}^2.$$

Hence,

$$\widehat{\lambda}_1(\widetilde{R}) - \frac{1}{2}(n-1) = M_n + \epsilon_n + O_p(n^{-1}). \tag{46}$$

Now, evaluating the term $\epsilon_n$ gives

$$\begin{aligned}\epsilon_n &= \frac{1}{n\lambda_1}\left\{ \sum_{\theta_i\theta_j=1, i\neq j} (\widetilde{R}_{ij}-a)^2 + \sum_{\theta_i\theta_j=-1} (\widetilde{R}_{ij}-b)^2 \right\} \\ &= \frac{1}{n\lambda_1}\left\{ \sum_{i\neq j} \widetilde{R}_{ij}^2 + \left(\frac{n^2}{2}-n\right)a^2 + \frac{n^2b^2}{2} - 2a \sum_{\theta_i\theta_j=1, i\neq j} \widetilde{R}_{ij} - 2b \sum_{\theta_i\theta_j=-1} \widetilde{R}_{ij} \right\}.\end{aligned} \tag{47}$$

When $E_1F_2 = 1/2$, then $a = b = 1/2 + O(n^{-1})$ holds from Eq. (42). Substituting these values into Eq. (47) gives

$$\epsilon_n = 2\sigma_n^2 + O_p(n^{-1}).$$

Therefore, rewriting Eq. (46) gives

$$\widehat{\lambda}_1(\widetilde{R}) - \frac{1}{2}(n-1) - 2\sigma_n^2 = M_n + O_p(n^{-1}). \tag{48}$$

In particular, the random term $M_n$ controls the behavior of $\widehat{\lambda}_1(\widetilde{R})$. To understand the asymptotic behavior of $\widehat{\lambda}_1(\widetilde{R})$, we proceed with moment calculations quantifying the properties of $M_n$.

According to Lemma 4, for $1 \leq k \leq n$, when $1 \leq i \neq j \leq n$, it holds that

$$\mathrm{cov}(\Gamma_{ki}, \Gamma_{kj}) = O(N^{-1}). \tag{49}$$

Computing the expectation of $M_n$ using Eq. (49) gives

$$E(M_n) = \frac{1}{n\lambda_1}\sum_{k=1}^{n}\sum_{i\neq j}\mathrm{cov}(\Gamma_{ki},\Gamma_{kj}) = O(n^{-1}).$$

Next, the second moment has the form

$$E(M_n^2) = \frac{1}{n^2\lambda_1^2}\sum_{k,i\neq j}\sum_{K,I\neq J}E(\Gamma_{ki}\Gamma_{kj}\Gamma_{KI}\Gamma_{KJ}).$$

By viewing the underlying set $V$ of $\{i,j,k,I,J,K\}$ as the node set of a graph and the subscript pairs $E=\{\{k,i\},\{k,j\},\{K,I\},\{K,J\}\}$ as edges, the summation can be analyzed by counting multigraphs $G=(V,E)$ where $V\subset [\![n]\!]$. In particular, graph counting techniques are used extensively in the proof of Lemma 8 where Eq. (77) gives

$$\sum_{k,i\neq j}\sum_{K,I\neq J}E(\Gamma_{ki}\Gamma_{kj}\Gamma_{KI}\Gamma_{KJ}) = 2\sum_{i,j,k\text{ distinct}}E(\Gamma_{ki}^2\Gamma_{kj}^2)+O(n^2).$$

We directly apply the above equation to the calculation of $E(M_n^2)$ and provide an abbreviated derivation below, since the full derivation is provided in the proof of Lemma 8. Namely, here

$$\begin{aligned}
&E(M_n^2)\\
&=\frac{1}{n^2\lambda_1^2}\sum_{k,i\neq j}\sum_{K,I\neq J}E(\Gamma_{ki}\Gamma_{kj}\Gamma_{KI}\Gamma_{KJ})\\
&=\frac{1}{n^2\lambda_1^2}\left\{2\sum_{i,j,k\text{ distinct}}E(\Gamma_{ki}^2\Gamma_{kj}^2)+O(n^2)\right\}\\
&=\frac{1}{n^2\lambda_1^2}\left\{2\sum_{i,j,k\text{ distinct}}E(\Gamma_{ki}^2)E(\Gamma_{kj}^2)+O(n^2)\right\} \qquad (50)\\
&=\frac{1}{n^2\lambda_1^2}\left[2\left\{n\left(\frac{n}{2}-1\right)\left(\frac{n}{2}-2\right)\sigma_a^4+\frac{n^2}{2}\left(\frac{n}{2}-1\right)\sigma_b^4+n^2\left(\frac{n}{2}-1\right)\sigma_a^2\sigma_b^2\right\}\right]+O(n^{-2})\\
&=\frac{2}{n}(\sigma_a^2+\sigma_b^2)^2+O(n^{-2})\\
&=\frac{1}{8n}\left(\frac{1}{6}+2E_1F_2\times E_2F_1\right)^2+O(n^{-2}),
\end{aligned}$$

where the third equality follows from Lemma 3 and the last equality uses the values of $\sigma_a^2$ and $\sigma_b^2$ given in Eq. (42). When $E_1F_2=1/2$, direct computation gives

$$E(M_n^2)=\widetilde{\sigma}_n^2+O(n^{-2}).$$

Having established that $E(M_n)=O(n^{-1})$ and $E(M_n^2)=\widetilde{\sigma}_n^2+O(n^{-2})$, it remains to study the higher moments of $M_n$ in order to establish asymptotic normality.

For every positive integer $l$, the $l$-th moment of $M_n$ has the property that

$$(n\lambda_1)^l E(M_n^l) = E\left(\sum_{k_1}\sum_{i_1\neq j_1}\cdots\sum_{k_l}\sum_{i_l\neq j_l}\Gamma_{k_1i_1}\Gamma_{k_1j_1}\cdots\Gamma_{k_li_l}\Gamma_{k_lj_l}\right).$$

By viewing the underlying set of $\{i_1, j_1, k_1, \ldots, i_l, j_l, k_l\}$, denoted as $V$, as the node set of a graph and the set of subscript pairs $E = \{\{k_1, i_1\}, \{k_1, j_1\}, \ldots, \{k_l, j_l\}\}$ as the edge set, the summation on the right-hand side of the above equation can be analyzed by counting multigraphs $G = (V, E)$ on $V \subset [\![n]\!]$, where $G$ consists of $l$ chains, each of length two. To reiterate, calculating $E(M_n^l)$ relies on analyzing the corresponding graph, as discussed in the proof of Lemma 8.

When $l$ is even, by referring to the proof of Lemma 8, the $l$-th moment has the property that

$$\begin{aligned}
&(n\lambda_1)^l E(M_n^l)\\
&\quad= E\left(\sum_{k_1}\sum_{i_1\neq j_1}\cdots\sum_{k_l}\sum_{i_l\neq j_l}\Gamma_{k_1 i_1}\Gamma_{k_1 j_1}\cdots\Gamma_{k_l i_l}\Gamma_{k_l j_l}\right)\\
&\quad= 2^{l/2}(l-1)!!\sum_{i_1,j_1,k_1,\ldots,k_{l/2}\text{ all distinct}} E(\Gamma^2_{k_1 i_1}\Gamma^2_{k_1 j_1}\cdots\Gamma^2_{k_{l/2} i_{l/2}}\Gamma^2_{k_{l/2} j_{l/2}}) + O(n^{3l/2-1}) \qquad (51)\\
&\quad= 2^{l/2}(l-1)!!\sum_{i_1,j_1,k_1,\ldots,k_{l/2}\text{ all distinct}} E(\Gamma^2_{k_1 i_1})E(\Gamma^2_{k_1 j_1})\cdots E(\Gamma^2_{k_{l/2} i_{l/2}})E(\Gamma^2_{k_{l/2} j_{l/2}})\\
&\qquad\quad + O(n^{3l/2-1}),
\end{aligned}$$

where the third equality follows from Lemma 3.

In the product term $E(\Gamma^2_{k_1 i_1})E(\Gamma^2_{k_1 j_1})\cdots E(\Gamma^2_{k_{l/2} i_{l/2}})E(\Gamma^2_{k_{l/2} j_{l/2}})$, each component $E(\Gamma^2_{k_s i_s})$ for $s = 1, \ldots, l/2$ can either be $\sigma_a^2$ or $\sigma_b^2$ depending on its subscript pair $(k_s, i_s)$. Specifically, if $\theta_{k_s}\theta_{i_s} = 1$, then $E(\Gamma^2_{k_s i_s}) = \sigma_a^2$; otherwise, $E(\Gamma^2_{k_s i_s}) = \sigma_b^2$. For example, given $k_1 \in [\![n]\!]$, it holds that

$$\left|\left\{i_1 : E(\Gamma^2_{k_1 i_1}) = \sigma_a^2\right\}\right| = n/2 - 1,$$

and

$$\left|\left\{i_1 : E(\Gamma^2_{k_1 i_1}) = \sigma_b^2\right\}\right| = n/2.$$

In words, if $k_1$ is chosen arbitrarily from $[\![n]\!]$, then there are $n/2 - 1$ choices of $i_1$ to make $E(\Gamma^2_{k_1 i_1})$ equal to $\sigma_a^2$ and $n/2$ choices of $i_1$ to make $E(\Gamma^2_{k_1 i_1})$ equal to $\sigma_b^2$. The same statement also holds for $E(\Gamma^2_{k_s i_s})$, with $s = 2, \ldots, l/2$ and $E(\Gamma^2_{k_s j_s})$ with $s = 1, \ldots, l/2$.

Suppose that in the product term $E(\Gamma^2_{k_1 i_1})E(\Gamma^2_{k_1 j_1})\cdots E(\Gamma^2_{k_{l/2} i_{l/2}})E(\Gamma^2_{k_{l/2} j_{l/2}})$ there are $m$ components equal to $\sigma_a^2$ and $l - m$ components equal to $\sigma_b^2$. Let

$$\begin{aligned}
S_m = \big\{&(k_1, i_1, j_1, \ldots, k_{l/2}, i_{l/2}, j_{l/2}) :\\
&E(\Gamma^2_{k_1 i_1})E(\Gamma^2_{k_1 j_1})\cdots E(\Gamma^2_{k_{l/2} i_{l/2}})E(\Gamma^2_{k_{l/2} j_{l/2}}) = \sigma_a^{2m}\sigma_b^{2(l-m)},\\
&k_1, i_1, j_1, \ldots, k_{l/2}, i_{l/2}, j_{l/2}\text{ are all distinct}\big\}.
\end{aligned}$$

A generalization of the above counting argument yields

$$|S_m| = n^{l/2} \times \left(\frac{n}{2}\right)^m \times \left(\frac{n}{2}\right)^{l-m} + O(n^{3l/2-1}).$$

Consequently,

$$\sum_{i_1,j_1,k_1,\ldots,k_{l/2}\text{ all distinct}} E(\Gamma^2_{k_1i_1})E(\Gamma^2_{k_1j_1})\cdots E(\Gamma^2_{k_{l/2}i_{l/2}})E(\Gamma^2_{k_{l/2}j_{l/2}})$$

$$\begin{aligned} &= \sum_{m=0}^{l}\binom{l}{m}\sigma_a^{2m}\sigma_b^{2(l-m)}\times|S_m| \\ &= \sum_{m=0}^{l}\binom{l}{m}\sigma_a^{2m}\sigma_b^{2(l-m)}\times\left(\frac{n}{2}\right)^m\times\left(\frac{n}{2}\right)^{l-m}\times n^{l/2}+O(n^{3l/2-1}) \\ &= \left(\frac{\sigma_a^2+\sigma_b^2}{2}\right)^l\times n^{3l/2}+O(n^{3l/2-1}). \end{aligned} \tag{52}$$

Now, applying the values in Eq. (42) to Eq. (52) yields

$$\sum_{i_1,j_1,k_1,\ldots,k_{l/2}\text{ all distinct}} E(\Gamma^2_{k_1i_1})E(\Gamma^2_{k_1j_1})\cdots E(\Gamma^2_{k_{l/2}i_{l/2}})E(\Gamma^2_{k_{l/2}i_{l/2}}) = \sigma_n^{2l}n^{3l/2}+O(n^{3l/2-1}).$$

By applying this equation to Eq. (51), we have that when $l$ is even,

$$E(M_n)^l = \widetilde{\sigma}_n^l(l-1)!!+O(n^{-l/2-1}).$$

When $l$ is odd, the discussion in the proof of Lemma 8 still applies here and gives

$$E(M_n^l) = O(n^{-l/2-1/2}).$$

Thus, we obtain

$$\lim_{n\to\infty} E(\widetilde{\sigma}_n^{-1}M_n)^l = \begin{cases}(l-1)!! & \text{if } l \text{ is even,}\\ 0 & \text{if } l \text{ is odd,}\end{cases}$$

which matches the moments of the standard normal distribution. From Billingsley (1995, Theorem 30.1 and Theorem 30.2), it follows that as $n \to \infty$,

$$\widetilde{\sigma}_n^{-1}M_n \to N(0,1) \qquad \text{in distribution.}$$

Hence, from Eq. (48), when $E_1F_2 = 1/2$, in the large-data limit,

$$T_n(\widetilde{R}) = \widetilde{\sigma}_n^{-1}\left\{\widehat{\lambda}_1(\widehat{R})-2^{-1}(n-1)-2\sigma_n^2\right\} \to N(0,1) \qquad \text{in distribution.}$$

This finishes the proof for the asymptotic normality of $T_n(\widetilde{R})$ when $E_1F_2 = 1/2$.

Next, we prove the stated claim for $T_n(\widetilde{R})$ under alternative hypotheses. Recall Eq. (46) and the definitions of $M_n$ and $\epsilon_n$ above, namely

$$\widehat{\lambda}_1(\widetilde{R})-2^{-1}(n-1) = M_n+\epsilon_n+O_p(n^{-1}).$$

Applying Eq. (42) to Eq. (47) and the fact that $E(M_n) = O(n^{-1})$ yields

$$E(M_n+\epsilon_n) = \frac{1}{4}\left(\frac{1}{6}+2E_1F_2\times E_2F_1\right)+O(n^{-1}). \tag{53}$$

Next, for ease of presentation but with slight abuse of notation, we define the quantities

$$\mathrm{cov}_{(a,a)} = E(\Gamma_{ij}\Gamma_{i'j'}), \qquad \theta_i\theta_j = \theta_{i'}\theta_{j'} = 1,\ \ \{i,j\}\neq\{i',j'\},$$

$$\mathrm{cov}_{(b,b)} = E(\Gamma_{ij}\Gamma_{i'j'}), \qquad \theta_i\theta_j = \theta_{i'}\theta_{j'} = -1,\ \ \{i,j\}\neq\{i',j'\},$$

and

$$\text{cov}_{(a,b)} = E(\Gamma_{ij}\Gamma_{i'j'}), \qquad \theta_i\theta_j \times \theta_{i'}\theta_{j'} = -1, \;\; \{i,j\} \neq \{i',j'\}.$$

The term $\sum_{i\neq j} \widetilde{R}_{ij}^2$ in Eq. (47) is a constant, thus the variance of $\epsilon_n$ can be expressed as

$$\begin{aligned}
\text{var}(\epsilon_n) &= \frac{4}{n^2\lambda_1^2}\text{var}\left(a \sum_{\theta_i\theta_j=1, i\neq j} \widetilde{R}_{ij} + b \sum_{\theta_i\theta_j=-1} \widetilde{R}_{ij}\right) \\
&= \frac{4}{n^2\lambda_1^2} E\left\{a \sum_{\theta_i\theta_j=1, i\neq j} (\widetilde{R}_{ij} - a) + b \sum_{\theta_i\theta_j=-1} (\widetilde{R}_{ij} - b)\right\}^2 \\
&= \frac{4}{n^2\lambda_1^2} E\left(a \sum_{\theta_i\theta_j=1, i\neq j} \Gamma_{ij} + b \sum_{\theta_i\theta_j=-1} \Gamma_{ij}\right)^2 \\
&= \frac{4}{n^2\lambda_1^2} E\left\{a^2\left(\sum_{\theta_i\theta_j=1, i\neq j} \Gamma_{ij}\right)^2 + b^2\left(\sum_{\theta_i\theta_j=-1} \Gamma_{ij}\right)^2\right. \\
&\qquad \left. +2ab \sum_{\theta_{i'}\theta_{j'}=-1} \sum_{\theta_i\theta_j=1, i\neq j} \Gamma_{ij}\Gamma_{i'j'}\right\} \\
&= \frac{4}{n^2\lambda_1^2}\left\{a^2\left(\frac{n^2}{2} - n\right)\left(\sigma_a^2 + a^2\right) + a^2\left(\frac{n^2}{2} - n\right)\left(\frac{n^2}{2} - n - 1\right)\text{cov}_{(a,a)}\right. \\
&\qquad \left. + \frac{b^2n^2}{2}(\sigma_b^2 + b^2) + \frac{b^2n^2}{2}\left(\frac{n^2}{2} - 1\right)\text{cov}_{(b,b)} + abn^2\left(\frac{n^2}{2} - n\right)\text{cov}_{(a,b)}\right\}.
\end{aligned}$$

Lemma 4 ensures that $\text{cov}(a,a)$, $\text{cov}(b,b)$, and $\text{cov}(a,b)$ all decay as $O(n^{-2})$. Therefore, simplifying the above variance calculation gives

$$\text{var}(\epsilon_n) = O(n^{-2}).$$

Recalling that Eq. (50) shows

$$E(M_n^2) = \frac{1}{8n}\left(\frac{1}{6} + 2E_1F_2 \times E_2F_1\right)^2 + O(n^{-2}),$$

thus it follows that

$$\begin{aligned}
\text{var}(M_n + \epsilon_n) &= \text{var}(M_n) + \text{var}(\epsilon_n) + 2\text{cov}(M_n, \epsilon_n) \\
&\leq \text{var}(M_n) + \text{var}(\epsilon_n) + 2\left\{\text{var}(M_n) \times \text{var}(\epsilon_n)\right\}^{1/2} \\
&= \frac{1}{8n}\left(\frac{1}{6} + 2E_1F_2 \times E_2F_1\right)^2 + O(n^{-3/2}).
\end{aligned} \tag{54}$$

Combining Eq. (53) and Eq. (54) with Eq. (46) yields

$$\widehat{\lambda}_1(\widetilde{R}) - 2^{-1}(n-1) = \frac{1}{4}\left(\frac{1}{6} + 2E_1F_2 \times E_2F_1\right) + O_p(n^{-1/2}).$$

In particular,

$$\widetilde{\sigma}_n^{-1}\left\{\widehat{\lambda}_1(\widetilde{R})-2^{-1}(n-1)-2\sigma_n^2\right\}=\widetilde{\sigma}_n^{-1}\left\{\frac{1}{4}\left(\frac{1}{6}+2E_1F_2\times E_2F_1\right)-2\sigma_n^2+O_p(n^{-1/2})\right\}$$
$$=\widetilde{\sigma}_n^{-1}\left\{\frac{1}{2}\left(E_1F_2\times E_2F_1-\frac{1}{4}\right)+O_p(n^{-1/2})\right\}$$
$$=-32^{-1/2}\times\sigma_n^{-2}n^{1/2}\left(E_1F_2-\frac{1}{2}\right)^2+O_p(1).$$

Hence, under sequences of alternatives for which $|E_1^{(n)}F_2^{(n)}-1/2|\gg n^{-1/4}$, it holds that

$$|T_n(\widetilde{R})|=\widetilde{\sigma}_n^{-1}\left|\widehat{\lambda}_1(\widetilde{R})-2^{-1}(n-1)-2\sigma_n^2\right|\to\infty$$

in probability as $n\to\infty$. This concludes the proof of Proposition 2. □

*Proof of Proposition 3.* Starting with Eq. (41), we have

$$\widehat{\lambda}_1-\lambda_1=u_1^{\mathrm{T}}\Gamma u_1+\frac{u_1^{\mathrm{T}}\Gamma^2u_1}{\lambda_1}+O_p(n^{-1}),$$

where $\widehat{\lambda}_1$ is the leading eigenvalue of $\widetilde{R}+\mathrm{diag}(\Theta\widetilde{B}\Theta^{\mathrm{T}})$ and $\lambda_1$ is the leading eigenvalue of $\Theta\widetilde{B}\Theta^{\mathrm{T}}$ with corresponding unit norm eigenvector $u_1$. Here, the leading eigenvector has the form $u_1=(x1_{n_1}^{\mathrm{T}},y1_{n-n_1}^{\mathrm{T}})^{\mathrm{T}}$. Denote

$$a=(\Theta\widetilde{B}\Theta^{\mathrm{T}})_{ij},\ \text{for } i,j \text{ satisfying } l_il_j=1, i\neq j,$$

and

$$b=(\Theta\widetilde{B}\Theta^{\mathrm{T}})_{ij},\ \text{for } i,j \text{ satisfying } l_il_j=0, i\neq j.$$

From $(\Theta\widetilde{B}\Theta^{\mathrm{T}})u_1=\lambda_1u_1$, we obtain the system of equations

$$\begin{cases}\lambda_1x=axn_1+by(n-n_1)\\ \lambda_1y=bxn_1+by(n-n_1).\end{cases}$$

When $a\neq b$, under the setting of Eq. (11) in the main text, there are only two non-zero eigenvalues of $\Theta\widetilde{B}\Theta^{\mathrm{T}}$. As such, $\lambda_1$ can be obtained by solving the above system of equations, yielding

$$\lambda_1=\frac{1}{2}\left[nb+n_1(a-b)+\{n^2b^2+2n_1(2n_1-n)b(a-b)+n_1^2(a-b)^2\}^{1/2}\right],$$

since

$$x=\frac{(n-n_1)b}{\{(n-n_1)(\lambda_1-n_1a)^2+n_1(n-n_1)^2b^2\}^{1/2}},$$

$$y=\frac{\lambda_1-n_1a}{\{(n-n_1)(\lambda_1-n_1a)^2+n_1(n-n_1)^2b^2\}^{1/2}}.$$

Direct computation shows that

$$a=\frac{1}{N+1}\left[\frac{n_1(n_1-1)}{2}\times\frac{1}{2}+\left\{N-\frac{n_1(n_1-1)}{2}\right\}\times E_1F_2+\frac{1}{2}\right],$$

$$b = \frac{1}{N+1}\left[\frac{n_1(n_1-1)}{2} \times E_2F_1 + \left\{N - \frac{n_1(n_1-1)}{2}\right\} \times \frac{1}{2} + \frac{1}{2}\right],$$

hence

$$a - b = E_1F_2 - 1/2 + O(n^{-2}).$$

Assuming $n_1 = o(n)$, let

$$z = \frac{2n_1(2n_1 - n)b(a-b) + n_1^2(a-b)^2}{n^2b^2},$$

and let $f(z) = (1+z)^{1/2}$. Then, $\lambda_1$ can be expressed as

$$\lambda_1 = \frac{1}{2}\left\{nb + n_1(a-b) + f(z)nb\right\}.$$

By viewing $\lambda_1$ as a function of $z = O\{n_1(a-b)/(nb)\} = o(1)$, taking a Taylor series expansion around $z = 0$ yields

$$\begin{aligned}
f(z) &= f(0) + f'(0)z + \frac{1}{2}f^{(2)}(0)z^2 + \frac{1}{6}f^{(3)}(0)z^3 + O(z^4)\\
&= 1 + \frac{1}{2}z - \frac{1}{8}z^2 + \frac{1}{16}z^3 + O(z^4)\\
&= 1 + \frac{2n_1(2n_1-n)b(a-b) + n_1^2(a-b)^2}{2n^2b^2} - \frac{\{2n_1(2n_1-n)b(a-b) + n_1^2(a-b)^2\}^2}{8n^4b^4}\\
&\qquad + \frac{\{2n_1(2n_1-n)b(a-b) + n_1^2(a-b)^2\}^3}{16n^6b^6} + O\left\{\frac{n_1^4(a-b)^4}{n^4b^4}\right\}\\
&= 1 + \frac{n_1(2n_1-n)(a-b)}{n^2b} + \frac{n_1^2(a-b)^2}{2n^2b^2} - \frac{n_1^2(2n_1-n)^2(a-b)^2}{2n^4b^2} - \frac{n_1^3(2n_1-n)(a-b)^3}{2n^4b^3}\\
&\qquad + \frac{n_1^3(2n_1-n)^3(a-b)^3}{2n^6b^3} + O\left\{\frac{n_1^4(a-b)^4}{n^4b^4}\right\}\\
&= 1 - \frac{n_1(a-b)}{nb} + \frac{2n_1^2(a-b)}{n^2b} + \frac{2n_1^3(a-b)^2}{n^3b^2} + O\left\{\frac{n_1^4(a-b)^2}{n^4b^2}\right\}.
\end{aligned}$$

Hence,

$$\begin{aligned}
\lambda_1 &= \frac{1}{2}\left\{nb + n_1(a-b) + f(z)nb\right\}\\
&= nb + \frac{n_1^2(a-b)}{n} + \frac{n_1^3(a-b)^2}{n^2b} + O\left\{\frac{n_1^4(a-b)^2}{n^3b}\right\}.
\end{aligned} \tag{55}$$

From Weyl's inequality, necessarily

$$|\widehat{\lambda}_1(\widetilde{R}) - \widehat{\lambda}_1| \le \max(a, b). \tag{56}$$

Applying Eq. (41) and Eq. (56) to the definition of the test statistic yields

$$\begin{aligned}
&\widetilde{\sigma}_n^{-1}\left\{\widehat{\lambda}_1(\widetilde{R}) - 2^{-1}(n-1) - 2\sigma_n^2\right\}\\
&\quad= \widetilde{\sigma}_n^{-1}\left\{\lambda_1 + u_1^{\mathrm{T}}\Gamma u_1 + \frac{u_1^{\mathrm{T}}\Gamma^2 u_1}{\lambda_1} - 2^{-1}(n-1) - 2\sigma_n^2 + O_p(1)\right\}.
\end{aligned} \tag{57}$$

Lemma 5 and Lemma 6 ensure that $u_1^{\mathrm{T}}\Gamma u_1 = O_p(1)$ and $u_1^{\mathrm{T}}\Gamma^2 u_1/\lambda_1 = O_p(1)$. So, further rewriting Eq. (57) using Eq. (55) gives

$$\begin{aligned}
T_n(\widetilde{R}) &= \widetilde{\sigma}_n^{-1}\left\{\widehat{\lambda}_1(\widetilde{R}) - 2^{-1}(n-1) - 2\sigma_n^2\right\} \\
&= \widetilde{\sigma}_n^{-1}\left\{\lambda_1 + u_1^{\mathrm{T}}\Gamma u_1 + \frac{u_1^{\mathrm{T}}\Gamma^2 u_1}{\lambda_1} - 2^{-1}(n-1) - 2\sigma_n^2 + O_p(1)\right\} \\
&= \widetilde{\sigma}_n^{-1}\left[n\left(b - \frac{1}{2}\right) + \frac{n_1^2(a-b)}{n} + \frac{n_1^3(a-b)^2}{n^2 b} + O\left\{\frac{n_1^4(a-b)^2}{n^3 b}\right\}\right. \\
&\qquad \left. - 2\sigma_n^2 + O_p(1)\right] \\
&= \widetilde{\sigma}_n^{-1}\left[\frac{n_1^3(E_1F_2 - 1/2)^2}{n^2/2 - n_1^2(E_1F_2 - 1/2)}\right. \\
&\qquad \left. + O\left\{\frac{n_1^4(E_1F_2 - 1/2)^2}{n^3/2 - nn_1^2(E_1F_2 - 1/2)}\right\} + O_p(1)\right].
\end{aligned}$$

Thus, if

$$\frac{n_1^3(E_1F_2 - 1/2)^2}{n^2 - 2n_1^2(E_1F_2 - 1/2)} \gg 1,$$

which holds under sequences of alternatives for which $|E_1^{(n)}F_2^{(n)} - 1/2| \gg n/n_1^{3/2}$ with $n_1 = o(n)$, then

$$|T_n(\widetilde{R})| = \widetilde{\sigma}_n^{-1}\left|\widehat{\lambda}_1(\widetilde{R}) - 2^{-1}(n-1) - 2\sigma_n^2\right| \to \infty$$

in probability as $n \to \infty$. This concludes the proof of Proposition 3. □

## Details for variance transition from dependence to independence

Define $\Gamma_k = \widetilde{R}_k - E(\widetilde{R}_k)$ as in the main text. From the definition of $\widetilde{R}_k$, it holds that $E\{(\Gamma_k)_{ij}\} = 0$, $\mathrm{var}\{(\Gamma_k)_{ij}\} = 1/12 - 1/\{6(N_k+1)\}$, and

$$\mathrm{var}(u_1^{\mathrm{T}}\Gamma_k u_1) = \mathrm{var}\left[\frac{2}{n} \times \left\{\sum_{p=1}^{N_k}(\Gamma_k)_p - \sum_{p=i_1}^{i_k}(\Gamma_k)_p\right\}\right] = 4n^{-2} \times \mathrm{var}\left\{\sum_{p=i_1}^{i_k}(\Gamma_k)_p\right\},$$

where $(\Gamma_k)_p$ denotes $p/(N_k+1)$, and $i_1, \ldots, i_k$ are randomly sampled without replacement from $\{1, \ldots, N_k\}$. This setup yields the variance equation

$$\mathrm{var}\left\{\sum_{p=i_1}^{i_k}(\Gamma_k)_p\right\} = \frac{k}{12} - \frac{k}{6(N_k+1)} - \frac{k(k-1)}{12(N_k+1)} = \frac{kN}{12(N+k+1)}.$$

Consequently, $\mathrm{var}(u_1^{\mathrm{T}}\Gamma_k u_1) = O\{k(N+k)^{-1}\}$. Similar to $\widehat{\lambda}_1(\widetilde{R})$, the variance of $\widehat{\lambda}_1(\widetilde{R}_k)$ is bounded from below by $\max\{\mathrm{var}(u_1^{\mathrm{T}}\Gamma_k u_1), \mathrm{var}(u_1^{\mathrm{T}}\Gamma_k^2 u_1/\lambda_1)\}$. The proof of Lemma 6 guarantees that $\mathrm{var}(u_1^{\mathrm{T}}\Gamma_k^2 u_1/\lambda_1) = O(n^{-1})$, so if $k(N+k)^{-1} = \Omega(n^{-1})$, then $\mathrm{var}\{\widehat{\lambda}_1(\widetilde{R}_k)\} = O\{k(N+$

$k)^{-1}\}$, otherwise $\text{var}\{\widehat{\lambda}_1(\widetilde{R}_k)\} = O(n^{-1})$. Notably, when $k \to \infty$, the off-diagonal entry distribution of $\widetilde{R}_k$ converges to that of $U$.

## ADDITIONAL PROOFS

This section provides proofs for the statements appearing in the first section of this supplementary material document.

*Proof of Lemma 1.* See Bai & Silverstein (2010, Corollary A.41). □

*Proof of Lemma 2.* See Billingsley (2013, Chapter 1). □

*Proof of Lemma 3.* We shall use a random vector of length $\sum_{k=1}^{l} \delta_k$, written as

$$(s_1^1, \dots, s_1^{\delta_1}, s_2^1, \dots, s_2^{\delta_2}, \dots, s_l^{\delta_l}),$$

to denote the subscripts of $\sum_{k=1}^{l} \delta_k$ arbitrary elements from $\{a_i\}_{1 \le i \le N}$. Each $s_i^j$ can range from 1 to $N$, hence we shall write

$$(s_1^1, \dots, s_1^{\delta_1}, \dots, s_l^{\delta_l}) \in [\![N]\!]^{\sum_{k=1}^{l} \delta_k}.$$

With this notation, rewriting $E(R_{i_1}^{\delta_1} \cdots R_{i_l}^{\delta_l})$ using indicator functions gives

$$\begin{aligned}
&E(R_{i_1}^{\delta_1} \cdots R_{i_l}^{\delta_l}) \\
&= E\left[\left\{\sum_{s_1=1}^{N} \mathbb{I}(a_{s_1} \le a_{i_1})\right\}^{\delta_1} \left\{\sum_{s_2=1}^{N} \mathbb{I}(a_{s_2} \le a_{i_2})\right\}^{\delta_2} \cdots \left\{\sum_{s_l=1}^{N} \mathbb{I}(a_{s_l} \le a_{i_l})\right\}^{\delta_l}\right] \\
&= E\left[\left\{\sum_{s_1^1=1}^{N} \cdots \sum_{s_1^{\delta_1}=1}^{N} \mathbb{I}(a_{s_1^1} \le a_{i_1}) \cdots \mathbb{I}(a_{s_1^{\delta_1}} \le a_{i_1})\right\}\right. \\
&\qquad \left. \cdots \left\{\sum_{s_l^1=1}^{N} \cdots \sum_{s_l^{\delta_l}=1}^{N} \mathbb{I}(a_{s_l^1} \le a_{i_l}) \cdots \mathbb{I}(a_{s_l^{\delta_l}} \le a_{i_l})\right\}\right].
\end{aligned} \tag{58}$$

Let $L = \{i_1, \dots, i_l\}$, and define the set $\bar{S}$ as

$$\bar{S} = \left\{(s_1^1, \dots, s_1^{\delta_1}, \dots, s_l^{\delta_l}) : s_i^j \in [\![N]\!] \backslash L, \;\; s_p^* \text{and } s_q^* \text{ are distinct when } p \ne q\right\},$$

where $s_p^*$ stands for $s_p^j$ with arbitrary $j = 1, \dots, \delta_p$. In words, $\bar{S}$ is the subset of $[\![N]\!]^{\sum_{k=1}^{l} \delta_k}$ in which every $\bar{s} \in \bar{S}$ has the following properties:

Entries with nonidentical subscripts are distinct.
No entries take values from $L$.

As such, the set complement $\bar{S}^c = [\![N]\!]^{\sum_{k=1}^{l} \delta_k} \backslash \bar{S}$ has the property

$$\left|\bar{S}^c\right| = O\left[\max\left\{\left(\sum_{k=1}^{l} \delta_k\right)^2 N^{\sum_{k=1}^{l} \delta_k - 1}, \left(\sum_{k=1}^{l} \delta_k\right) l N^{\sum_{k=1}^{l} \delta_k - 1}\right\}\right], \tag{59}$$

because, for any $\bar{s} \in \bar{S}^c$, at least two entries of $\bar{s}$ are the same or at least one entry belongs to $L$. As a result, proceeding with Eq. (58), we have

$$
\begin{aligned}
&E(R_{i_1}^{\delta_1} \cdots R_{i_l}^{\delta_l}) \\
&= E\left\{ \sum_{\bar{s}\in\bar{S}} \mathbb{I}(a_{s_1^1} \le a_{i_1}) \cdots \mathbb{I}(a_{s_l^{\delta_l}} \le a_{i_l}) + \sum_{\bar{s}\in\bar{S}^c} \mathbb{I}(a_{s_1^1} \le a_{i_1}) \cdots \mathbb{I}(a_{s_l^{\delta_l}} \le a_{i_l}) \right\} \\
&= E\left\{ \sum_{\bar{s}\in\bar{S}} \mathbb{I}(a_{s_1^1} \le a_{i_1}) \cdots \mathbb{I}(a_{s_l^{\delta_l}} \le a_{i_l}) \right\} + O\left(N^{\sum_{k=1}^l \delta_k - 1}\right) \\
&= \sum_{\bar{s}=(s_1^1,\ldots,s_l^{\delta_l})\in\bar{S}} E\left\{ \mathbb{I}(a_{s_1^1} \le a_{i_1}) \cdots \mathbb{I}(a_{s_1^{\delta_1}} \le a_{i_1}) \right\} \cdots E\left\{ \mathbb{I}(a_{s_l^1} \le a_{i_l}) \cdots \mathbb{I}(a_{s_l^{\delta_l}} \le a_{i_l}) \right\} \\
&\qquad + O\left(N^{\sum_{k=1}^l \delta_k - 1}\right) \\
&= \sum_{\bar{s}=(s_1^1,\ldots,s_l^{\delta_l})\in[\![N]\!]^{\sum_{k=1}^l \delta_k}} E\left\{ \mathbb{I}(a_{s_1^1} \le a_{i_1}) \cdots \mathbb{I}(a_{s_1^{\delta_1}} \le a_{i_1}) \right\} \times \cdots \\
&\qquad \times E\left\{ \mathbb{I}(a_{s_l^1} \le a_{i_l}) \cdots \mathbb{I}(a_{s_l^{\delta_l}} \le a_{i_l}) \right\} + O\left(N^{\sum_{k=1}^l \delta_k - 1}\right),
\end{aligned}
$$

where both the second and the last equality invoke Eq. (59). By writing $\widetilde{R}_k = R_k/(N+1)$, the above equation gives

$$
E(\widetilde{R}_{i_1}^{\delta_1} \cdots \widetilde{R}_{i_l}^{\delta_l}) = E(\widetilde{R}_{i_1}^{\delta_1}) \cdots E(\widetilde{R}_{i_l}^{\delta_l}) + O(N^{-1}). \tag{60}
$$

Recall that $\Gamma_k$ is the normalized rank statistic $\widetilde{R}_k - E(\widetilde{R}_k)$. We therefore have that

$$
E(\Gamma_{i_1}^{\delta_1}\Gamma_{i_2}^{\delta_2} \cdots \Gamma_{i_l}^{\delta_l}) = E\left[ \{\widetilde{R}_{i_1} - E(\widetilde{R}_{i_1})\}^{\delta_1} \cdots \{\widetilde{R}_{i_l} - E(\widetilde{R}_{i_l})\}^{\delta_l} \right].
$$

Rewriting the above equation and applying Eq. (60) yields

$$
\begin{aligned}
E(\Gamma_{i_1}^{\delta_1}\Gamma_{i_2}^{\delta_2}\cdots\Gamma_{i_l}^{\delta_l}) &= E\left\{\sum_{k_1=0}^{\delta_1}\binom{\delta_1}{k_1}\widetilde{R}_{i_1}^{k_1}\{-E(\widetilde{R}_{i_1})\}^{\delta_1-k_1}\cdots\sum_{k_l=0}^{\delta_l}\binom{\delta_l}{k_l}\widetilde{R}_{i_l}^{k_l}\{-E(\widetilde{R}_{i_l})\}^{\delta_l-k_l}\right\}\\
&= E\left\{\sum_{k_1=0}^{\delta_1}\cdots\sum_{k_l=0}^{\delta_l}\binom{\delta_1}{k_1}\cdots\binom{\delta_l}{k_l}\{-E(\widetilde{R}_{i_1})\}^{\delta_1-k_1}\right.\\
&\qquad\left.\cdots\{-E(\widetilde{R}_{i_l})\}^{\delta_l-k_l}\widetilde{R}_{i_1}^{k_1}\cdots\widetilde{R}_{i_l}^{k_l}\right\}\\
&= \sum_{k_1=0}^{\delta_1}\cdots\sum_{k_l=0}^{\delta_l}\binom{\delta_1}{k_1}\cdots\binom{\delta_l}{k_l}\{-E(\widetilde{R}_{i_1})\}^{\delta_1-k_1}\\
&\qquad\cdots\{-E(\widetilde{R}_{i_l})\}^{\delta_l-k_l}E(\widetilde{R}_{i_1}^{k_1})\cdots E(\widetilde{R}_{i_l}^{k_l})+O(N^{-1})\\
&= E\left\{\sum_{k_1=0}^{\delta_1}\binom{\delta_1}{k_1}\widetilde{R}_{i_1}^{k_1}\{-E(\widetilde{R}_{i_1})\}^{\delta_1-k_1}\right\}\\
&\qquad\cdots E\left\{\sum_{k_l=0}^{\delta_l}\binom{\delta_l}{k_l}\widetilde{R}_{i_l}^{k_l}\{-E(\widetilde{R}_{i_l})\}^{\delta_l-k_l}\right\}+O(N^{-1})\\
&= E(\Gamma_{i_1}^{\delta_1})E(\Gamma_{i_2}^{\delta_2})\cdots E(\Gamma_{i_l}^{\delta_l})+O(N^{-1}),
\end{aligned}
$$

i.e.,

$$
\left|E(\Gamma_{i_1}^{\delta_1}\Gamma_{i_2}^{\delta_2}\cdots\Gamma_{i_l}^{\delta_l}) - E(\Gamma_{i_1}^{\delta_1})E(\Gamma_{i_2}^{\delta_2})\cdots E(\Gamma_{i_l}^{\delta_l})\right| = O(N^{-1}).
$$

This completes the proof of Lemma 3. □

*Proof of Lemma 4.* When $m = 0$, namely when $\delta_t > 1$ for all $t \in \{1, \ldots, l\}$, applying the observation $|\Gamma_i| \leq 1$ for $1 \leq i \leq N$ implies

$$
\left|E(\Gamma_{i_1}^{\delta_1}\cdots\Gamma_{i_l}^{\delta_l})\right| \leq 1.
$$

Hence, the special case $m = 0$ in Lemma 4 is proved.

When $m > 0$, namely when there exists at least one $t \in \{1, \ldots, l\}$, such that $\delta_t = 1$, the remaining proof of Lemma 4 proceeds via a combinatorial argument. Without loss of generality, let $r = l - m$ and assume $\delta_t > 1$ for $t = 1, \ldots, r$, and $\delta_t = 1$ for $t = r + 1, \ldots, l$. Then,

$$
\left|E(\Gamma_{i_1}^{\delta_1}\cdots\Gamma_{i_l}^{\delta_l})\right| = \left|E(\Gamma_{i_1}^{\delta_1}\cdots\Gamma_{i_r}^{\delta_r}\Gamma_{i_{r+1}}\cdots\Gamma_{i_l})\right|.
$$

Further, rewriting the above expression in terms of indicator functions gives

$$\left|E(\Gamma_{i_1}^{\delta_1}\cdots\Gamma_{i_r}^{\delta_r}\Gamma_{i_{r+1}}\cdots\Gamma_{i_l})\right| = \left|\frac{1}{(N+1)^{\delta_1+\cdots+\delta_r+(l-r)}}\right.$$
$$E\left(\left[\sum_{j_1=1}^{N}\mathbb{I}(a_{j_1}\le a_{i_1}) - E\left\{\sum_{j_1=1}^{N}\mathbb{I}(a_{j_1}\le a_{i_1})\right\}\right]^{\delta_1}\right.$$
$$\cdots\left[\sum_{j_r=1}^{N}\mathbb{I}(a_{j_r}\le a_{i_r}) - E\left\{\sum_{j_r=1}^{N}\mathbb{I}(a_{j_r}\le a_{i_r})\right\}\right]^{\delta_r}$$
$$\left[\sum_{j_{r+1}=1}^{N}\mathbb{I}(a_{j_{r+1}}\le a_{i_{r+1}}) - E\left\{\sum_{j_{r+1}=1}^{N}\mathbb{I}(a_{j_{r+1}}\le a_{i_{r+1}})\right\}\right]$$
$$\left.\left.\cdots\left[\sum_{j_l=1}^{N}\mathbb{I}(a_{j_l}\le a_{i_l}) - E\left\{\sum_{j_l=1}^{N}\mathbb{I}(a_{j_l}\le a_{i_l})\right\}\right]\right)\right|.$$

Let $H(j_k, i_k) = \mathbb{I}(a_{j_k} \le a_{i_k}) - E\{\mathbb{I}(a_{j_k} \le a_{i_k})\}$. Using this notation and rewriting the above expression yields

$$\begin{aligned}
&(N+1)^{\delta_1+\cdots+\delta_r+(l-r)}\left|E(\Gamma_{i_1}^{\delta_1}\cdots\Gamma_{i_r}^{\delta_r}\Gamma_{i_{r+1}}\cdots\Gamma_{i_l})\right| \\
&= \left|E\left[\left\{\sum_{j_1}H(j_1,i_1)\right\}^{\delta_1}\cdots\left\{\sum_{j_r}H(j_r,i_r)\right\}^{\delta_r}\left\{\sum_{j_{r+1}}H(j_{r+1},i_{r+1})\right\}\cdots\left\{\sum_{j_l}H(j_l,i_l)\right\}\right]\right| \\
&= \left|E\left\{\sum_{j_1^1}H(j_1^1,i_1)\sum_{j_1^2}H(j_1^2,i_1)\cdots\sum_{j_1^{\delta_1}}H(j_1^{\delta_1},i_1)\sum_{j_2^1}H(j_2^1,i_2)\cdots\sum_{j_l}H(j_l,i_l)\right\}\right| \\
&= \left|E\left\{\sum_{j_1^1}\sum_{j_1^2}\cdots\sum_{j_1^{\delta_1}}\sum_{j_2^1}\cdots\sum_{j_l}H(j_1^1,i_1)H(j_1^2,i_1)\cdots H(j_1^{\delta_1},i_1)H(j_2^1,i_2)\cdots H(j_l,i_l)\right\}\right|.
\end{aligned} \tag{61}$$

By viewing the underlying set of subscripts $\{i_1, j_1^1, j_1^2, \ldots, j_1^{\delta_1}, \ldots, j_l\}$, denoted as $V$, as the node set of a graph and the pairs $E = \{\{j_1^1, i_1\}, \{j_1^2, i_1\}, \ldots, \{j_l, i_l\}\}$ as the edge set, the above summation involves multigraphs $G = (V, E)$ wherein nodes $j_p^* \in V, p = 1, \ldots, l$ are chosen arbitrarily from $[\![N]\!]$.

Let the random vector of length $\sum_{t=1}^{r}\delta_t + (l-r)$, denoted $\bar{s} = (j_1^1, j_1^2, \ldots, j_l)$, represent the nodes $j_p^* \in V, p = 1, \ldots, l$, and denote

$$\bar{S} = \left\{(j_1^1, \ldots, j_l) \in [\![N]\!]^{\sum_{t=1}^{r}\delta_t+(l-r)} : \text{ for all } k \in \{r+1, \ldots, l\}, \{j_k, i_k\} \text{ is not an isolated edge}\right\}.$$

It follows that the set complement is

$$\begin{aligned}\bar{S}^C &= [\![N]\!]^{\sum_{t=1}^r \delta_t + (l-r)} \backslash \bar{S} \\ &= \Big\{ (j_1^1, \dots, j_l) \in [\![N]\!]^{\sum_{t=1}^r \delta_t + (l-r)} : \\ &\qquad \text{there exists } k \in \{r+1, \dots, l\}, \text{ such that } \{j_k, i_k\} \text{ is an isolated edge} \Big\}.\end{aligned}$$

Using this notation, rewriting Eq. (61) gives

$$\begin{aligned}\text{Eq. (61)} = &\Bigg| E\left\{ \sum_{\bar{s}\in\bar{S}} H(j_1^1, i_1) H(j_1^2, i_1) \cdots H(j_1^{\delta_1}, i_1) H(j_2^1, i_2) \cdots H(j_l, i_l) \right\} \\ &\quad + E\left\{ \sum_{\bar{s}\in\bar{S}^C} H(j_1^1, i_1) H(j_1^2, i_1) \cdots H(j_1^{\delta_1}, i_1) H(j_2^1, i_2) \cdots H(j_l, i_l) \right\} \Bigg| \\ = &\left| E\left\{ \sum_{\bar{s}\in\bar{S}} H(j_1^1, i_1) H(j_1^2, i_1) \cdots H(j_1^{\delta_1}, i_1) H(j_2^1, i_2) \cdots H(j_l, i_l) \right\} \right| \\ \le &\sum_{\bar{s}\in\bar{S}} \left| E\left\{ H(j_1^1, i_1) H(j_1^2, i_1) \cdots H(j_1^{\delta_1}, i_1) H(j_2^1, i_2) \cdots H(j_l, i_l) \right\} \right|.\end{aligned} \tag{62}$$

The second equality holds because, if there exists a $k \in \{r+1, \dots, l\}$ such that $\{j_k, i_k\}$ is an isolated edge, then the corresponding component term $H(j_k, i_k)$ is independent of the other component terms. Thus, the property that $E\{H(j_k, i_k)\} = 0$ reduces the whole term to zero. Given that $|H(j, i)| \le 1$, the overall bound in Eq. (62) depends only on the cardinality of the set $\bar{S}$.

Next, by the enumerative counting argument provided below, we shall establish that there exists a constant $C \equiv C(l, r, \delta_1, \dots, \delta_r)$ such that

$$|\bar{S}| \le C N^{\delta_1 + \cdots + \delta_r + (l-r)/2}.$$

To this end, consider the following:

1) Denote

$$\bar{S}_d = \left\{ \bar{s} \in \bar{S} : \text{the number of distinct entries in } \bar{s} \text{ is } d \right\}.$$

Since every $\bar{s}$ has $\sum_{t=1}^r \delta_t + l - r$ entries, the number of ways to divide these entries into $d$ groups is upper-bounded by $d^{\sum_{t=1}^r \delta_t + l - r}$. Then, each group chooses a value from $[\![N]\!]$ while ensuring the $d$ values are distinct. Thus,

$$|\bar{S}_d| \le d^{\sum_{t=1}^r \delta_t + l - r} N^d.$$

2) We now discuss the maximum value of $d$.

Observe that compared to two unconnected edges, two connected edges have at least one fewer distinct node. For example, if $\{j_1^1, i_1\}$ and $\{j_{r+1}, i_{r+1}\}$ do not have common nodes, since $i_1$ and $i_{r+1}$ are fixed, these two edges contribute 2 distinct nodes ($j_1^1$ and $j_{r+1}$) that can take values freely from $[\![N]\!]$, namely 2 distinct entries in $\bar{s}$. Once $\{j_1^1, i_1\}$ and $\{j_{r+1}, i_{r+1}\}$ connect, since $i_1$ and $i_{r+1}$ are not arbitrary, there are at most three possibilities: $j_1^1 = i_{r+1}$, $j_{r+1} = i_1$, or

$j_1^1 = j_{r+1}$. All three possibilities result in one fewer distinct unfixed node. Particularly, after connecting, there is only 1 unfixed node in $\{j_1^1, i_1\}$ and $\{j_{r+1}, i_{r+1}\}$, i.e., they only contribute 1 distinct entry in $\bar{s}$.

According to the previous discussion, each time we connect two edges, the number of distinct entries in $\bar{s}$ is reduced by 1. Starting with an $\bar{s} \in \bar{S}^c$, where all $\sum_{t=1}^r \delta_t + l - r$ entries are distinct from each other, we calculate the minimum number of edge connections needed to transform $\bar{s}$ into an element of $\bar{S}$. By definition, for all $k \in \{r+1, \ldots, l\}$, the edge $\{j_k, i_k\}$ is not isolated, so each $\{j_k, i_k\}$ must be connected to at least one other edge. To ensure that none of the edges are isolated, when $l - r$ is even, at least $(l-r)/2$ edge connections must be made (pairing the edges in $\{\{j_k, i_k\}, k = r+1, \ldots, l\}$), and when $l - r$ is odd, at least $(l-r+1)/2$ edge connections are required.

Starting with $\sum_{t=1}^r \delta_t + l - r$ distinct entries, after at least $(l-r)/2$ connecting steps, $\bar{s}$ will have at most $\sum_{t=1}^r \delta_t + (l-r)/2$ distinct entries. Therefore, for every $\bar{s} \in \bar{S}$, there are at most $\sum_{t=1}^r \delta_t + (l-r)/2$ distinct entries, i.e., $d \leq \sum_{t=1}^r \delta_t + (l-r)/2$.

3) Summarizing the above counting arguments, by definition, there exists a positive constant $C$ satisfying

$$C \equiv C(\delta_1 + \cdots + \delta_l) < \left(\sum_{t=1}^{l} \delta_t\right)^{\sum_{t=1}^l \delta_t + 1}$$

such that

$$|\bar{S}| = \sum_{d=1}^{\sum_{t=1}^r \delta_t + (l-r)/2} \left|\bar{S}_d\right| \leq CN^{\delta_1 + \cdots + \delta_r + (l-r)/2}.$$

Since $|H(j,i)| \leq 1$, we have

$$\text{Eq. (62)} \leq \sum_{\bar{s} \in \bar{S}} 1 \leq CN^{\delta_1 + \cdots + \delta_r + (l-r)/2}.$$

Thus,

$$\left|E(\Gamma_{i_1}^{\delta_1} \cdots \Gamma_{i_l}^{\delta_l})\right| \leq CN^{-m/2}.$$

This concludes the proof of Lemma 4. □

*Proof of Lemma 5.* By direct computation and linearity of expectation, it holds that

$$E(x^{\mathrm{T}} \Gamma^l y) = \sum_i \sum_j x_i y_j E(\Gamma^l)_{ij} = \sum_i x_i y_i E(\Gamma^l)_{ii} + \sum_{i \neq j} x_i y_j E(\Gamma^l)_{ij}, \tag{63}$$

where given a pair of indices $(i, j)$, $1 \leq i, j \leq n$, we have

$$E(\Gamma^l)_{ij} = \sum_{1 \leq i \neq i_1, i_1 \neq i_2, \ldots, i_{l-1} \neq j \leq n} E(\Gamma_{ii_1} \Gamma_{i_1 i_2} \cdots \Gamma_{i_{l-1} j}).$$

By viewing the underlying set of $\{i, i_1, i_2, \ldots, i_{l-1}, j\}$, denoted as $V$, as the node set of a graph, and $E = \{\{i, i_1\}, \{i_1, i_2\}, \ldots, \{i_{l-1}, j\}\}$ as the edge set, the above summation involves multigraphs $G = (V, E)$ wherein nodes $i_p \in V$, $p = 1, \ldots, l-1$ take values from $[\![N]\!]$. For each pair of $i$ and

$j$, $G$ is a chain of length $l$ with fixed beginning and ending nodes. The following proof employs a combinatorial graph enumeration strategy to bound $E(x^{\mathrm{T}}\Gamma^l y)$.

When $i \neq j$, for each multigraph $G$, let $s$ denote the number of distinct edges in $E$, and let $m$ denote the number of single edges in $E$. Then, there are $s - m$ edges that have multiplicity of at least two. Since the total number of edges is $l$, we have

$$m + 2(s - m) \leq l. \tag{64}$$

Further, it will be useful to write

$$G(s, m) = \{\text{Graphs with } s \text{ distinct edges and } m \text{ single edges}\}.$$

The graphs can be divided into two groups according to the number of distinct edges $s$. Namely,

$$\begin{aligned}\sum_{1\leq i\neq i_1, i_1\neq i_2,\ldots,i_{l-1}\neq j\leq n} E(\Gamma_{ii_1}\Gamma_{i_1i_2}\cdots\Gamma_{i_{l-1}j}) &= \sum_{s\leq l/2}\sum_{m}\sum_{G(s,m)} E(\Gamma_{ii_1}\Gamma_{i_1i_2}\cdots\Gamma_{i_{l-1}j}) \\ &\quad + \sum_{s>l/2}\sum_{m}\sum_{G(s,m)} E(\Gamma_{ii_1}\Gamma_{i_1i_2}\cdots\Gamma_{i_{l-1}j}).\end{aligned} \tag{65}$$

Given the structure of $G$, the number of non-isomorphic graphs to $G$ is upper bounded by $l^l$. Since $l$ is assumed to be fixed and $|\Gamma_{ij}| \leq 1$, the bound of the above equation only depends on the number of possible node choices.

First, consider the first term on the right-hand side of Eq. (65). Any connected graph with $s$ distinct edges necessarily has at most $s + 1$ distinct nodes. Therefore, when $l$ is an even positive integer, each chain in the first term on the right-hand side of Eq. (65) has at most $l/2 + 1$ distinct nodes. Since here $i, j$ are taken to be fixed, the number of ways of choosing nodes from $[\![n]\!]$ for this term is $O(n^{l/2-1})$. When $l$ is odd, $s$ is at most $(l - 1)/2$, and it can be similarly established that the number of ways to choose nodes from $[\![n]\!]$ for this term is $O\{n^{(l-1)/2-1}\}$.

In summary,

$$\sum_{s\leq l/2}\sum_{m}\sum_{G(s,m)} E(\Gamma_{ii_1}\Gamma_{i_1i_2}\cdots\Gamma_{i_{l-1}j}) = \begin{cases} O(n^{l/2-1}) & \text{when } l \text{ is even,} \\ O\{n^{(l-1)/2-1}\} & \text{when } l \text{ is odd.}\end{cases}$$

Next, consider the second term on the right-hand side of Eq. (65). Similarly, since the nodes $i, j$ are taken to be fixed in this term, a chain with $s$ distinct edges has at most $O(n^{s-1})$ ways of choosing nodes. From Lemma 4, for $G \in G(s, m)$, the expectation with subscripts corresponding to $G$ has the property

$$E(\Gamma_{ii_1}\Gamma_{i_1i_2}\cdots\Gamma_{i_{l-1}j}) = O(n^{-m}).$$

For each fixed $s$, Eq. (64) restricts the possible values of $m$ between $2s - l$ and $l$. By combining this with the expectation bound, we obtain that when $l$ is even, there exists $C_l \geq 0$ such that

$$\sum_{s>l/2}\sum_{m}\sum_{G(s,m)} E(\Gamma_{ii_1}\Gamma_{i_1i_2}\cdots\Gamma_{i_{l-1}j}) \leq \sum_{s=l/2+1}^{l}\sum_{m=2s-l}^{l} l^l n^{s-1} \times C_l n^{-m} = O(n^{l/2-1}).$$

In contrast, when $l$ is odd, there exists $C_l \geq 0$ such that

$$\sum_{s>l/2}\sum_{m}\sum_{G(s,m)} E(\Gamma_{ii_1}\Gamma_{i_1i_2}\cdots\Gamma_{i_{l-1}j}) \leq \sum_{s=(l+1)/2}^{l}\sum_{m=2s-l}^{l} l^l n^{s-1} \times C_l n^{-m} = O\{n^{(l-1)/2-1}\}.$$

Summarizing the above discussion, for $i \neq j$, when $i, j$ are fixed, then

$$E(\Gamma^l)_{ij} = \sum_{i \neq i_1, i_1 \neq i_2, \ldots, i_{l-1} \neq j} E(\Gamma_{ii_1}\Gamma_{i_1i_2}\cdots\Gamma_{i_{l-1}j}) = \begin{cases} O(n^{l/2-1}) & \text{when } l \text{ is even,} \\ O\{n^{(l-1)/2-1}\} & \text{when } l \text{ is odd.} \end{cases} \quad (66)$$

We now consider the case $i = j$. When $i = j$ and $i, j$ are fixed, each chain in $G(s, m)$ has at most $s + 1$ distinct nodes. Given that $i = j$ is fixed, there are at most $n^s$ possible ways to select the remaining nodes. Aside from node selection, the analysis is similar to the case when $i \neq j$ and is therefore omitted here. The upshot is that

$$E(\Gamma^l)_{ii} = \sum_{i \neq i_1, i_1 \neq i_2, \ldots, i_{l-1} \neq i} E(\Gamma_{ii_1}\Gamma_{i_1i_2}\cdots\Gamma_{i_{l-1}i}) = \begin{cases} O(n^{l/2}) & \text{when } l \text{ is even,} \\ O\{n^{(l-1)/2}\} & \text{when } l \text{ is odd.} \end{cases} \quad (67)$$

Since $x_i y_i \leq (x_i^2 + y_i^2)/2$, combining Eq. (63), Eq. (66) and Eq. (67) yields,

$$\begin{aligned} E(x^{\mathrm{T}}\Gamma^l y) &\leq \sum_i \frac{1}{2}\left(x_i^2 + y_i^2\right) E(\Gamma^l)_{ii} + \sum_{i \neq j} \frac{1}{2}\left(x_i^2 + y_j^2\right) E(\Gamma^l)_{ij} \\ &= \begin{cases} O(n^{l/2}) & \text{when } l \text{ is even,} \\ O\{n^{(l-1)/2}\} & \text{when } l \text{ is odd.} \end{cases} \end{aligned}$$

This completes the proof of Lemma 5. □

*Proof of Lemma 6.* This proof proceeds by computing the order of the variance of $x^{\mathrm{T}}\Gamma^l y - E(x^{\mathrm{T}}\Gamma^l y)$ and then obtaining the stated bound using Chebyshev's inequality.

Firstly, direct computation shows

$$\begin{aligned} &E\{x^{\mathrm{T}}\Gamma^l y - E(x^{\mathrm{T}}\Gamma^l y)\}^2 \\ &= \sum_{1 \leq i_1, \ldots, i_{l+1} \leq n} \sum_{1 \leq j_1, \ldots, j_{l+1} \leq n} E\left[\left\{x_{i_1}\Gamma_{i_1i_2}\cdots\Gamma_{i_li_{l+1}}y_{i_{l+1}} - E(x_{i_1}\Gamma_{i_1i_2}\cdots\Gamma_{i_li_{l+1}}y_{i_{l+1}})\right\}\right. \\ &\quad \left.\times\left\{x_{j_1}\Gamma_{j_1j_2}\cdots\Gamma_{j_lj_{l+1}}y_{j_{l+1}} - E(x_{j_1}\Gamma_{j_1j_2}\cdots\Gamma_{j_lj_{l+1}}y_{j_{l+1}})\right\}\right] \\ &= \sum_{1 \leq i_1, \ldots, i_{l+1} \leq n} \sum_{1 \leq j_1, \ldots, j_{l+1} \leq n} x_{i_1}x_{j_1}y_{i_{l+1}}y_{j_{l+1}} \left\{E(\Gamma_{i_1i_2}\cdots\Gamma_{i_li_{l+1}}\Gamma_{j_1j_2}\cdots\Gamma_{j_lj_{l+1}})\right. \\ &\quad \left.-E(\Gamma_{i_1i_2}\cdots\Gamma_{i_li_{l+1}})E(\Gamma_{j_1j_2}\cdots\Gamma_{j_lj_{l+1}})\right\}. \end{aligned}$$

By viewing the underlying set of the subscripts $\{i_1, i_2, \ldots, i_{l+1}, j_1, \ldots, j_{l+1}\}$, denoted as $V$, as the node set of a graph, and $E = \{\{i_1, i_2\}, \ldots, \{j_l, j_{l+1}\}\}$ as the edge set, the above summation can be analyzed via the multigraph $G = (V, E)$, where $V \subset [\![n]\!]$. Observe that $G$ is a graph consisting of two chains, each of length $l$.

The proof proceeds by analyzing different cases of graphs and establishing that

$$E\left\{x^{\mathrm{T}}\Gamma^l y - E(x^{\mathrm{T}}\Gamma^l y)\right\}^2 = O(n^{l-1}).$$

Now, given $m \in [\![2l]\!]$, we categorize the collection of graphs with $m$ single edges into four cases. For each case, we derive separate bounds for the corresponding summations. We then combine these bounds and sum over $m$ to obtain the final overall bound.

Denote

$$G(s, m) = \{\text{Graphs with } s \text{ distinct edges and } m \text{ single edges}\}.$$

Case 1: Denote $G_1 = \{G \in G(l,m): \text{ the two chains do not connect}\}$. According to Lemma 3, for each $G \in G_1$, the corresponding expectation has the property

$$\left|E(\Gamma_{i_1i_2}\cdots\Gamma_{i_li_{l+1}}\Gamma_{j_1j_2}\cdots\Gamma_{j_lj_{l+1}}) - E(\Gamma_{i_1i_2}\cdots\Gamma_{i_li_{l+1}})E(\Gamma_{j_1j_2}\cdots\Gamma_{j_lj_{l+1}})\right| = O(n^{-2}). \tag{68}$$

For notational simplicity, let $I_1$ and $I_2$ denote the first and last nodes of the first chain, and let $I_3$ and $I_4$ denote the first and last nodes of the second chain. The number of distinct nodes in a chain is at most one more than the number of distinct edges, hence a graph consisting of of two separate chains with a total of $l$ distinct edges has at most $l+2$ distinct nodes. Then, excluding $I_1, I_2, I_3, I_4$, there are $l-2$ nodes to be selected arbitrarily from $[\![n]\!]$. Similarly label these nodes as $I_5, \ldots, I_{l+2}$. Then, since a graph of two chains with a total of $2l$ edges has fewer than $(2l)^{2l}$ non-isomorphic graphs, using the Cauchy–Schwarz inequality and Eq. (68), an upper-bound of the summation of the corresponding expectations in this case is

$$\begin{aligned}
&\sum_{G_1} x_{i_1}x_{j_1}y_{i_{l+1}}y_{j_{l+1}}\left\{E(\Gamma_{i_1i_2}\cdots\Gamma_{i_li_{l+1}}\Gamma_{j_1j_2}\cdots\Gamma_{j_lj_{l+1}}) - E(\Gamma_{i_1i_2}\cdots\Gamma_{i_li_{l+1}})E(\Gamma_{j_1j_2}\cdots\Gamma_{j_lj_{l+1}})\right\}\\
&\qquad\le \sum_{I_1,\ldots,I_{l+2}} x_{I_1}y_{I_2}x_{I_3}y_{I_4}\times(2l)^{2l}\times O(n^{-2})\\
&\qquad\le \left(\sum_{I_1} x_{I_1}^2\right)^{1/2}\left(\sum_{I_2} y_{I_2}^2\right)^{1/2}\left(\sum_{I_3} x_{I_3}^2\right)^{1/2}\left(\sum_{I_4} y_{I_4}^2\right)^{1/2}\\
&\qquad\quad\times n^2\times n^{l-2}\times(2l)^{2l}\times O(n^{-2})\\
&\qquad= O(n^{l-2}).
\end{aligned}$$

Case 2: Denote $G_2 = \{G \in G(l,m): \text{ the two chains connect}\}$. Again, for notational simplicity, let $I_1$ and $I_2$ denote the first and last nodes of the first chain, and let $I_3$ and $I_4$ denote the first and last nodes of the second chain.

A connected graph with $l$ distinct edges has at most $l+1$ distinct nodes. Here, we label these distinct nodes $I_1, \ldots, I_{l+1}$ as in Case 1. Additionally, the definition of matrix $\Gamma$ yields

$$\left|E(\Gamma_{i_1i_2}\cdots\Gamma_{i_li_{l+1}}\Gamma_{j_1j_2}\cdots\Gamma_{j_lj_{l+1}}) - E(\Gamma_{i_1i_2}\cdots\Gamma_{i_li_{l+1}})E(\Gamma_{j_1j_2}\cdots\Gamma_{j_lj_{l+1}})\right| \le 1.$$

Hence, an upper bound for the summation of the corresponding expectations in this case is

$$\begin{aligned}
&\sum_{G_2} x_{i_1}x_{j_1}y_{i_{l+1}}y_{j_{l+1}}\left\{E(\Gamma_{i_1i_2}\cdots\Gamma_{i_li_{l+1}}\Gamma_{j_1j_2}\cdots\Gamma_{j_lj_{l+1}}) - E(\Gamma_{i_1i_2}\cdots\Gamma_{i_li_{l+1}})E(\Gamma_{j_1j_2}\cdots\Gamma_{j_lj_{l+1}})\right\}\\
&\qquad\le \sum_{I_1,\ldots,I_{l+1}} x_{I_1}y_{I_2}x_{I_3}y_{I_4}\times(2l)^{2l}\\
&\qquad\le \left(\sum_{I_1} x_{I_1}^2\right)^{1/2}\left(\sum_{I_2} y_{I_2}^2\right)^{1/2}\left(\sum_{I_3} x_{I_3}^2\right)^{1/2}\left(\sum_{I_4} y_{I_4}^2\right)^{1/2}\times n^2\times n^{l-3}\times(2l)^{2l}\\
&\qquad= O(n^{l-1}).
\end{aligned}$$

Case 3: Denote $G_3 = \bigcup\{G(s,m): s \le l-1\}$. If the two chains are separate, then the number of distinct nodes in the graph is at most $s+2$. Otherwise, it is at most $s+1$. Similar to the previous discussion, it holds that

$$\left|E(\Gamma_{i_1i_2}\cdots\Gamma_{i_li_{l+1}}\Gamma_{j_1j_2}\cdots\Gamma_{j_lj_{l+1}}) - E(\Gamma_{i_1i_2}\cdots\Gamma_{i_li_{l+1}})E(\Gamma_{j_1j_2}\cdots\Gamma_{j_lj_{l+1}})\right| \le 1,$$

so an upper-bound for the summation of the corresponding expectations in this case is

$$\sum_{G_3} x_{i_1}x_{j_1}y_{i_{l+1}}y_{j_{l+1}}\left\{E(\Gamma_{i_1i_2}\cdots\Gamma_{i_li_{l+1}}\Gamma_{j_1j_2}\cdots\Gamma_{j_lj_{l+1}}) - E(\Gamma_{i_1i_2}\cdots\Gamma_{i_li_{l+1}})E(\Gamma_{j_1j_2}\cdots\Gamma_{j_lj_{l+1}})\right\}$$
$$\leq \sum_{s=1}^{l-1}\sum_{I_1,\ldots,I_{s+2}} x_{I_1}y_{I_2}x_{I_3}y_{I_4}\times(2l)^{2l}$$
$$= O(n^{l-1}).$$

Case 4: Denote $G_4 = \bigcup\{G(s,m) : s \geq l+1\}$. For each $G \in G_4$, let $s_1$ and $s_2$ denote the number of single edges in chain 1 and chain 2, respectively. Then, $s_1 + s_2 \geq m$. Lemma 4 ensures that

$$\left|E(\Gamma_{i_1i_2}\cdots\Gamma_{i_li_{l+1}})\right| = O(n^{-s_1}),$$

$$\left|E(\Gamma_{j_1j_2}\cdots\Gamma_{j_lj_{l+1}})\right| = O(n^{-s_2}),$$

and

$$\left|E(\Gamma_{i_1i_2}\cdots\Gamma_{i_li_{l+1}}\Gamma_{j_1j_2}\cdots\Gamma_{j_lj_{l+1}})\right| = O(n^{-m}).$$

Therefore,

$$\left|E(\Gamma_{i_1i_2}\cdots\Gamma_{i_li_{l+1}}\Gamma_{j_1j_2}\cdots\Gamma_{j_lj_{l+1}}) - E(\Gamma_{i_1i_2}\cdots\Gamma_{i_li_{l+1}})E(\Gamma_{j_1j_2}\cdots\Gamma_{j_lj_{l+1}})\right| = O(n^{-m}).$$

A graph of two chains with $s$ distinct edges has at most $s+2$ distinct nodes, so we similarly bound the summation of the corresponding expectations in this case as

$$\sum_{G_4} x_{i_1}x_{j_1}y_{i_{l+1}}y_{j_{l+1}}\left\{E(\Gamma_{i_1i_2}\cdots\Gamma_{i_li_{l+1}}\Gamma_{j_1j_2}\cdots\Gamma_{j_lj_{l+1}}) - E(\Gamma_{i_1i_2}\cdots\Gamma_{i_li_{l+1}})E(\Gamma_{j_1j_2}\cdots\Gamma_{j_lj_{l+1}})\right\}$$
$$\leq \sum_{s=l+1}^{2l}\sum_{I_1,\ldots,I_{s+2}} x_{I_1}y_{I_2}x_{I_3}y_{I_4}\times(2l)^{2l}\times O(n^{-m})$$
$$= \sum_{s=l+1}^{2l} O(n^{s-m}). \tag{69}$$

Now, for each $G \in G_4$, there are a total of $2l$ edges. Eq. (64) in this case takes the form

$$m + 2(s-m) \leq 2l,$$

i.e.,

$$m \geq 2(s-l).$$

By definition, for each $G \in G_4$, it holds that $s \geq l+1$. Therefore, the above equation induces that $|G_4| > 0$ only when $m \geq 2$. The same inequality also ensures that $s - m \leq l - m/2$. Thus, we obtain that $s - m \leq l - 1$, and

$$\text{Eq. (69)} = O(n^{l-1}).$$

Summarizing Case 1 to Case 4 yields

$$
\begin{aligned}
E\{x^{\mathrm{T}}\Gamma^{l}y - E(x^{\mathrm{T}}\Gamma^{l}y)\}^{2} &= \sum_{m=0}^{2l}\sum_{t=1}^{4}\sum_{G_t} x_{i_1}x_{j_1}y_{i_{l+1}}y_{j_{l+1}}\left\{E(\Gamma_{i_1i_2}\cdots\Gamma_{i_li_{l+1}}\Gamma_{j_1j_2}\cdots\Gamma_{j_lj_{l+1}})\right.\\
&\qquad \left. -E(\Gamma_{i_1i_2}\cdots\Gamma_{i_li_{l+1}})E(\Gamma_{j_1j_2}\cdots\Gamma_{j_lj_{l+1}})\right\}\\
&= O(n^{l-1}),
\end{aligned}
$$

and so the stated claim holds by an application of Chebyshev's inequality. This completes the proof of Lemma 6. □

*Proof of Lemma 7.* As before, let $\widetilde{R}_{ij} = R_{ij}/(N+1)$ and write $\Gamma = \widetilde{R} - E(\widetilde{R})$. For $a_1, \ldots, a_N$, define the symmetric matrix $A$ with zero main diagonal such that $\mathrm{vech}_0(A) = (a_1, \ldots, a_N)^{\mathrm{T}}$. Let $g : \{(i,j), 1 \le i < j \le n\} \to [\![N]\!]$ be the map such that if $A_{ij} \sim F_d$, then $g(i,j) = d$. Further, let $F(A)$ denote the entry-wise transformation on $A$ such that

$$
F(A)_{ij} = \begin{cases} \sum_{i'<j'} F_{g(i',j')}(A_{ij})/(N+1) + 1/\{2(N+1)\} & \text{if } i \neq j,\\ 0 & \text{if } i = j. \end{cases}
$$

Using this notation, it follows from the triangle inequality that

$$
\|\widetilde{R} - E(\widetilde{R})\| = \|\widetilde{R} - F(A) + F(A) - E(\widetilde{R})\| \le \|\widetilde{R} - F(A)\| + \|F(A) - E(\widetilde{R})\|.
$$

By definition, $F(A)$ is a symmetric random matrix with independent and bounded entries, and $E\{F(A)\} = E(\widetilde{R})$. According to Chen et al. (2021, Theorem 3.4), there exists a constant $C > 0$, such that

$$
\mathrm{pr}\left(\|F(A) - E(\widetilde{R})\| > 5n^{1/2}\right) \le n\exp(-Cn). \tag{70}
$$

It remains to show that $\|\widetilde{R} - F(A)\| = O(n^{1/2})$ holds with high probability.

Fix a pair of $(i,j), i \neq j$, observe that

$$
\begin{aligned}
\left|\widetilde{R}_{ij} - F(A)_{ij}\right| &= \left|\frac{1}{N+1}\sum_{i'<j'}\left\{\mathbb{I}(A_{i'j'} \le A_{ij}) - F_{g(i',j')}(A_{ij})\right\} - \frac{1}{2(N+1)}\right|\\
&= \left|\frac{1}{N+1}\sum_{i'<j',\{i',j'\}\neq\{i,j\}}\left\{\mathbb{I}(A_{i'j'} \le A_{ij}) - E_{i'j'}\mathbb{I}(A_{i'j'} \le A_{ij})\right\}\right.\\
&\qquad \left. + \frac{1}{N+1}\left\{1/2 - F_{g(i,j)}(A_{ij})\right\}\right|\\
&\le \left|\frac{1}{N+1}\sum_{i'<j',\{i',j'\}\neq\{i,j\}}\left\{\mathbb{I}(A_{i'j'} \le A_{ij}) - E_{i'j'}\mathbb{I}(A_{i'j'} \le A_{ij})\right\}\right| + \frac{1}{2(N+1)},
\end{aligned} \tag{71}
$$

where $E_{i'j'}\mathbb{I}(A_{i'j'} \le A_{ij})$ denotes $\int \mathbb{I}(x \le A_{ij})\mathrm{d}F_{g(i',j')}(x)$ and is a function of $A_{ij}$. In particular,

$$
E\left[\sum_{i'<j',\{i',j'\}\neq\{i,j\}}\left\{\mathbb{I}(A_{i'j'} \le A_{ij}) - E_{i'j'}\mathbb{I}(A_{i'j'} \le A_{ij})\right\} \,\middle|\, A_{ij}\right] = 0.
$$

Fix $A_{ij} = x$, then $\mathbb{I}(A_{i'j'} \le x) - E_{i'j'}\mathbb{I}(A_{i'j'} \le x)$, $i' < j'$, $\{i', j'\} \ne \{i, j\}$ are bounded random variables independent of each other. From Bernstein's inequality (Vershynin, 2018, Theorem 2.8.4), it holds that

$$\mathrm{pr}\left[\left|\sum_{i'<j',\{i',j'\}\ne\{i,j\}} \left\{\mathbb{I}(A_{i'j'} \le x) - E_{i'j'}\mathbb{I}(A_{i'j'} \le x)\right\}\right| \ge \frac{N}{n^{1/2}}\right] \le 2\exp\left\{-\frac{N^2/(2n)}{\sigma^2(x) + N/(3n^{1/2})}\right\}, \tag{72}$$

where $\sigma^2(x) = \sum_{i'<j',\{i',j'\}\ne\{i,j\}} E_{i'j'}\left\{\mathbb{I}(A_{i'j'} \le x) - E_{i'j'}\mathbb{I}(A_{i'j'} \le x)\right\}^2 \le N$. Thus, combining Eq. (71) and Eq. (72) yields that for $n \ge 2$,

$$\begin{aligned}
&\mathrm{pr}\left\{\left|\widetilde{R}_{ij} - F(A)_{ij}\right| \ge n^{-1/2} + 2^{-1}(N+1)^{-1}\right\} \\
&\quad \le \mathrm{pr}\left[\left|\frac{1}{N+1}\sum_{i'<j',\{i',j'\}\ne\{i,j\}} \left\{\mathbb{I}(A_{i'j'} \le A_{ij}) - E_{i'j'}\mathbb{I}(A_{i'j'} \le A_{ij})\right\}\right| \ge n^{-1/2}\right] \\
&\quad \le \int \mathrm{pr}\left[\left|\sum_{i'<j',\{i',j'\}\ne\{i,j\}} \left\{\mathbb{I}(A_{i'j'} \le x) - E_{i'j'}\mathbb{I}(A_{i'j'} \le x)\right\}\right| \ge \frac{N+1}{n^{1/2}} \mid A_{ij} = x\right] \mathrm{d}F_{g(i,j)}(x) \\
&\quad \le \int 2\exp\left\{-\frac{N^2/(2n)}{\sigma^2(x) + N/(3n^{1/2})}\right\} \mathrm{d}F_{g(i,j)}(x) \\
&\quad \le 2\exp\left\{-\frac{N^2/(2n)}{N + N/(3n^{1/2})}\right\} \\
&\quad \le 2\exp(-n/10)\,.
\end{aligned} \tag{73}$$

Applying Eq. (73) to bound the Frobenius norm of $\widetilde{R} - F(A)$ yields that for $n \ge 2$,

$$\begin{aligned}
\mathrm{pr}\left(\|\widetilde{R} - F(A)\|_{\mathrm{F}} > n^{1/2}\right) &= \mathrm{pr}\left(\|\widetilde{R} - F(A)\|_{\mathrm{F}}^2 > n\right) \\
&\le \sum_{1\le i\ne j\le n} \mathrm{pr}\left(\left|\widetilde{R}_{ij} - F(A)_{ij}\right|^2 \ge \frac{1}{n-1}\right) \\
&\le \sum_{1\le i\ne j\le n} \mathrm{pr}\left\{\left|\widetilde{R}_{ij} - F(A)_{ij}\right| \ge n^{-1/2} + 2^{-1}(N+1)^{-1}\right\} \\
&\le 2n^2\exp(-n/10)\,.
\end{aligned} \tag{74}$$

By combining Eq. (74) and Eq. (70), there exists a universal constant $C_1 > 0$ such that

$$\begin{aligned}
\mathrm{pr}\left(\|\Gamma\| \ge 6n^{1/2}\right) &\le \mathrm{pr}\left(\|\widetilde{R} - F(A)\|_{\mathrm{F}} \ge n^{1/2}\right) + \mathrm{pr}\left(\|F(A) - E(\widetilde{R})\| \ge 5n^{1/2}\right) \\
&\le 2n^2\exp(-n/10) + \exp(-Cn) \\
&\le \exp(-C_1 n).
\end{aligned}$$

This completes the proof of Lemma 7. □

*Proof of Lemma 8.* Let $M_n = \sum_{k=1}^{n} N^{-1} \sum_{i\neq j} \Gamma_{ki}\Gamma_{kj}$. By direct computation, $u_1^{\mathrm{T}}\Gamma^2 u_1$ can be expanded in the manner

$$\begin{aligned} u_1^{\mathrm{T}}\Gamma^2 u_1 &= \frac{1}{n}\sum_{i=1}^{n}\sum_{j=1}^{n}\sum_{k=1}^{n}\Gamma_{ik}\Gamma_{kj} \\ &= \frac{1}{n}\sum_{k=1}^{n}\sum_{i\neq j}\Gamma_{ki}\Gamma_{kj} + \frac{1}{n}\sum_{k=1}^{n}\sum_{i=1}^{n}\Gamma_{ki}^2 \\ &= \frac{n-1}{2}M_n + \frac{2}{n}\sum_{i<j}\Gamma_{ij}^2 \\ &= \frac{n-1}{2}M_n + \frac{2}{n}\sum_{i=1}^{N}\left(\frac{i}{N+1} - \frac{1}{2}\right)^2 \\ &= \frac{n-1}{2}M_n + \frac{n-1}{12} + O(n^{-1}). \end{aligned}$$

In particular,

$$\frac{2}{n-1}\left\{u_1^{\mathrm{T}}\Gamma^2 u_1 - \frac{n-1}{12}\right\} = M_n + O(n^{-2}).$$

The proof idea is to establish asymptotic normality by matching the moments of $\widetilde{\sigma}_n^{-1}M_n$ with the moments of the standard normal distribution. To that end, first observe that

$$E(M_n) = E\left(\frac{2n}{N}\sum_{j<k}\Gamma_{ij}\Gamma_{ik}\right) = \frac{2n}{N}\binom{n-1}{2}\left\{-\frac{1}{12(N+1)}\right\} = -\frac{n-2}{6(N+1)}.$$

Next, consider

$$E(M_n^2) = \frac{1}{N^2}E\left(\sum_i\sum_{j\neq k}\Gamma_{ij}\Gamma_{ik}\right)^2 = \frac{1}{N^2}E\left(\sum_i\sum_{j\neq k}\sum_I\sum_{J\neq K}\Gamma_{ji}\Gamma_{ik}\Gamma_{JI}\Gamma_{IK}\right).$$

By viewing the underlying set $V$ of the subscripts $\{i, j, k, I, J, K\}$ as the node set of a graph and the pairs $E = \{\{j, i\}, \{i, k\}, \{J, I\}, \{I, K\}\}$ as edges, the above summation can be interpreted via multigraphs $G = (V, E)$ where $V \subset [\![n]\!]$. Observe that $G$ is a graph of two chains, each of length two.

Denote

$$G(d, s) = \{\text{Graphs with } d \text{ distinct nodes and } s \text{ single edges}\}.$$

According to Lemma 4, for $G \in G(d, s)$, the corresponding expectation satisfies

$$E\left(\Gamma_{ji}\Gamma_{ik}\Gamma_{JI}\Gamma_{IK}\right) = O(n^{-s}).$$

Since every such $G$ has 4 edges, the number of non-isomorphic graphs for $G$ is at most $4^4$. Additionally, each node in $V$ takes values from $[\![n]\!]$, so the number of ways to choose nodes for $G \in G(d, s)$ is at most $O(n^d)$. Therefore,

$$\sum_{G(d,s)} E(\Gamma_{ji}\Gamma_{ik}\Gamma_{JI}\Gamma_{IK}) = O(n^{d-s}),$$

and

$$N^2 E(M_n^2) = \sum_{d,s} \sum_{G(d,s)} E\left(\Gamma_{ji}\Gamma_{ik}\Gamma_{JI}\Gamma_{IK}\right) = O\left(\sum_{d,s} n^{d-s}\right).$$

Now, suppose $2 \le m \le 4$ is the number of distinct edges for a multigraph $G \in G(d,s)$. Since the number of distinct nodes in a connected graph is at most one more than the number of distinct edges, and there are at most two separate chains in $G$ (when $m = 4$, $d = 6$), we have

$$d \le \begin{cases} m+1 & \text{if } m \le 3, \\ m+2 & \text{if } m = 4. \end{cases} \tag{75}$$

Furthermore, Eq. (64) also applies here in the form

$$s + 2(m - s) \le 4. \tag{76}$$

Eq. (75) and Eq. (76) together yield

$$d - s \le 3.$$

Thus,

$$N^2 E(M_n^2) = O(n^3).$$

Next, we discuss the structure of the graphs in $G(d,s)$ with $d - s = 3$.

If the two chains $\{\{j,i\},\{i,k\}\}$ and $\{\{J,I\},\{I,K\}\}$ do not have common nodes and $j,i,k,J,I,K$ are all distinct, then $d = 6$, $s = 4$, and $d - s = 2$.

Starting with this graph, we shall gradually reduce the number of single edges $s$ and determine how this change affects the structure of the graph.

1) In the summation, we exclude the cases where $j = k$ and $J = K$. To reduce $s$ by 2, we need to connect the two chains and create one repeated edge. In this case, two distinct nodes are also removed, reducing $d$ by 2, and $d - s$ remains unchanged.

2) To reduce $s$ by 3, three edges out of the four should be identical. However, since $J \ne K$ and $j \ne k$, no graphs in the summation have the property $s = 1$.

3) To reduce $s$ by 4, we either pair the four edges two-by-two or make the four edges identical to each other. Again, because $J \ne K$ and $j \ne k$, the summation excludes the latter case. In the former case, $d = 3$, $s = 0$, and $d - s = 3$.

The above discussion shows that the graph with $d - s = 3$ has the property that $(i,j) = (I,J)$, $(i,k) = (I,K)$, or $(i,j) = (I,K)$, $(i,k) = (I,J)$. All other graphs have $d - s \le 2$. From this, we

decompose $E(M_n^2)$ into a leading order term and a residual term in the manner

$$
\begin{aligned}
&E(M_n^2)\\
&=\frac{1}{N^2}\left\{\sum_{i=I,j=J,k=K,j\neq k} E\left(\Gamma_{ji}\Gamma_{ik}\Gamma_{JI}\Gamma_{IK}\right)+\sum_{i=I,j=K,k=J,j\neq k} E\left(\Gamma_{ji}\Gamma_{ik}\Gamma_{JI}\Gamma_{IK}\right)+O(n^2)\right\}\\
&=\frac{1}{N^2}\left\{2\sum_{i,j,k \text{ distinct}} E(\Gamma_{ij}^2\Gamma_{ik}^2)+O(n^2)\right\}\\
&=\frac{1}{N^2}\left\{2\sum_{i,j,k \text{ distinct}} E(\Gamma_{ij}^2)E(\Gamma_{ik}^2)+O(n^2)\right\}\\
&=\frac{2n^3(\sigma_n^2)^2+O(n^2)}{N^2}\\
&=\widetilde{\sigma}_n^2+O(n^{-2}),
\end{aligned}
\tag{77}
$$

where the third equality invokes Lemma 3.

In what follows, we generalize the above discussion for arbitrary positive integer powers $l$. Consider

$$
N^l E(M_n^l)=E\left(\sum_{i_1}\sum_{j_1\neq k_1}\cdots\sum_{i_l}\sum_{j_l\neq k_l}\Gamma_{j_1i_1}\Gamma_{i_1k_1}\cdots\Gamma_{j_li_l}\Gamma_{i_lk_l}\right). \tag{78}
$$

Similarly, define the corresponding multigraph $G=(V,E)$, then $G$ consists of $l$ chains, each of length two.

We shall call the activity of overlaying two distinct edges an *action*. The number of distinct nodes and the number of single edges reduced by an action are the *parameters* of this action and are denoted as $(\Delta d, \Delta s)$. We call $r=\Delta s-\Delta d$ the *effective rate* of an action. For ease of discussion, let us call the activity of connecting nodes without overlaying edges a *non-action activity*. Similarly define $r$ for non-action activity, so it follows that non-action activity has $r<0$.

Starting with the graph where all nodes are distinct, we have $d=3l$, $s=2l$, and $d-s=l$. The corresponding expectations in this case satisfy

$$
\sum_{G(3l,2l)} E\left(\Gamma_{j_1i_1}\Gamma_{i_1k_1}\cdots\Gamma_{j_li_l}\Gamma_{i_lk_l}\right)=O(n^l).
$$

Suppose we take a total of $T$ activities sequentially, among which there are $t$ actions and $T-t$ non-action activities. Let $r_i, i=1,\ldots,t$ denote the effective rate of each action. Then, the resulting graphs have the property that $d-s\leq l+\sum_{i=1}^t r_i$. Let $G(T,r_1,\ldots,r_t)$ denote the collection of graphs resulting from the above sequence of activities. The expectation corresponding to the graphs after taking these activities is bounded in the manner

$$
\sum_{G(T,r_1,\ldots,r_t)} E\left(\Gamma_{j_1i_1}\Gamma_{i_1k_1}\cdots\Gamma_{j_li_l}\Gamma_{i_lk_l}\right)=O\left(n^{l+\sum_{i=1}^t r_i}\right).
$$

Observe that starting at $G(3l,2l)$, all possible graphs involved in the summation on the right-hand side of Eq. (78) can be reached by a sequence of actions and non-action activities. Additionally, since $G$ only has $2l$ edges, the total number of activities required to reach any of the possible

graphs is upper-bounded by a positive constant $C_l$. Thus, overall,

$$E\left(\sum_{i_1}\sum_{j_1\neq k_1}\cdots\sum_{i_l}\sum_{j_l\neq k_l}\Gamma_{j_1 i_1}\Gamma_{i_1 k_1}\cdots\Gamma_{j_l i_l}\Gamma_{i_l k_l}\right)$$
$$\leq \sum_{0\leq T\leq C_l}\sum_{t=0}^{T}\sum_{r_1,\ldots,r_t}\sum_{G(T,r_1,\ldots,r_t)} E\left(\Gamma_{j_1 i_1}\Gamma_{i_1 k_1}\cdots\Gamma_{j_l i_l}\Gamma_{i_l k_l}\right)$$
$$= O\left(\max_{t,r_1,\ldots,r_t} n^{l+\sum_{i=1}^{t} r_i}\right),$$

where the maximum on the right-hand side considers the sequence of actions that results in the largest summation $\sum_i r_i$.

For each action, the possible pairs $(\Delta d, \Delta s)$ with positive $\Delta s$ are as follows:

1) $(2, 2)$, i.e., (overlay two single edges with no common nodes);
2) $(1, 2)$, i.e., (overlay two single edges with one common node);
3) $(2, 1)$, i.e., (overlay one repeated edge and one single edge without common nodes);
4) $(1, 1)$, i.e., (overlay one repeated edge and one single edge with one common node).

Among the outlined actions, only the action of overlaying two single edges with one common node $(1, 2)$ has the effective rate $r > 0$. It follows that the resulting graphs from a sequence of actions with the most $(1, 2)$ actions reach the largest $\sum_i r_i$. However, since $j_p \neq k_p$ for all $p = 1, \ldots, l$, before an $(1, 2)$ action, at least one activity to connect two chains is needed in order to create common nodes. Among the activities that can connect two separate chains, the $(2, 2)$ action is the most efficient since other activities have $r < 0$.

Therefore, if conducting a sequence of $t$ actions, the strategy that produces the largest $\sum_{i=1}^{t} r_i$ is to conduct $t/2$ $(1, 2)$ and $t/2$ $(2, 2)$ actions in an alternating manner, starting with $(2, 2)$ followed by $(1, 2)$. Observe that one $(2, 2)$ action and one $(1, 2)$ action together reduce the number of single edges by 4. There are a total of $2l$ single edges in the starting state $G(3l, 2l)$. So, when $l$ is even, $t$ is at most $l$, while when $l$ is odd, $t$ is at most $(2l - 1)/2$.

Next, consider when $l$ is even. We discuss the resulting graph structure after conducting $l/2$ $(1, 2)$ actions and $l/2$ $(2, 2)$ actions in the above alternating manner. Recall that the state $G(3l, 2l)$ contains $l$ separate chains, each of length 2. For the first action in the sequence, we randomly select two of the $l$ chains and perform $(2, 2)$ action on them. For ease of presentation, denote the two selected chains $\{\{j, i\}, \{i, k\}\}$ and $\{\{J, I\}, \{I, K\}\}$ respectively. The $(2, 2)$ action can only do one of the following:

Connect $j$ and $J$ (or $k$ and $K$), $i$ and $I$ to overlay $\{j, i\}$ and $\{J, I\}$ (or $\{k, i\}$ and $\{K, I\}$). (I)

Connect $j$ and $K$ (or $k$ and $J$), $i$ and $I$ to overlay $\{j, i\}$ and $\{K, I\}$ (or $\{k, i\}$ and $\{J, I\}$). (II)

Connect $j$ and $I$ (or $k$ and $I$), $i$ and $J$ to overlay $\{j, i\}$ and $\{J, I\}$ (or $\{k, i\}$ and $\{J, I\}$). (III)

Connect $k$ and $I$ (or $j$ and $I$), $i$ and $K$ to overlay $\{k, i\}$ and $\{K, I\}$ (or $\{j, i\}$ and $\{K, I\}$). (IV)

Among them, the structure of the connected chains resulting from Eq. (III) and Eq. (IV) makes a follow-up $(1, 2)$ action impossible. Hence, the $(2, 2)$ action can either do Eq. (I) or Eq. (II). If it is Eq. (I), the following $(1, 2)$ then overlays $\{k, i\}$ and $\{K, I\}$ (or $\{j, i\}$ and $\{J, I\}$, respectively); on the other hand, if it is Eq. (II), the following $(1, 2)$ then overlays $\{k, i\}$ and $\{J, I\}$ (or $\{j, i\}$ and $\{K, I\}$, respectively). Upon finishing the first $(2, 2)$ action and first $(1, 2)$ action on one pair of randomly selected chains. We randomly choose two chains again from the remaining $l - 2$ chains

and conduct $(2,2)$ action and $(1,2)$ action on them similarly. This process will continue until the $l/2$-th $(2,2)$ action and $l/2$-th $(1,2)$ are completed. Finally, the resulting graph structure will be $G(3l/2,0)$, i.e.,

$$\max_{t,r_i,\ldots,r_t} n^{l+\sum_{i=1}^t r_i} = O(n^{3l/2}).$$

Observe that all other strategies only lead to at most $O(n^{3l/2-1})$ contribution. It follows that

$$\begin{aligned} &E\left(\sum_{i_1}\sum_{j_1\neq k_1}\cdots\sum_{i_l}\sum_{j_l\neq k_l}\Gamma_{j_1i_1}\Gamma_{i_1k_1}\cdots\Gamma_{j_li_l}\Gamma_{i_lk_l}\right)\\ &\quad=\sum_{G(3l/2,0)} E\left(\Gamma_{j_1i_1}\Gamma_{i_1k_1}\cdots\Gamma_{j_li_l}\Gamma_{i_lk_l}\right)+O(n^{3l/2-1}). \end{aligned} \tag{79}$$

Now, we further evaluate the term

$$\sum_{G(3l/2,0)} E(\Gamma_{j_1i_1}\Gamma_{i_1k_1}\cdots\Gamma_{j_li_l}\Gamma_{i_lk_l}).$$

According to the sequence of actions described above, for every $G\in G(3l/2,0)$, there are a total of $l/2$ separate chains, among which every chain is formed by two paired original chains conducting $(2,2)$ and $(1,2)$ in order. There are

$$\frac{l!}{2^{l/2}(l/2)!} = (l-1)!!$$

ways to pair the $l$ chains two by two. Additionally, as previously discussed, for each pair out of $l/2$ pairs, there are two ways to connect the nodes, thus contributing a factor of $2^{l/2}$. Therefore, combining the above counting argument with Lemma 3, it can be deduced that

$$\begin{aligned} &\sum_{G(3l/2,0)} E\left(\Gamma_{j_1i_1}\Gamma_{i_1k_1}\cdots\Gamma_{j_li_l}\Gamma_{i_lk_l}\right)\\ &\quad= 2^{l/2}(l-1)!!\sum_{i_1,j_1,k_1,\ldots,k_{l/2}\text{ all distinct}} E(\Gamma_1^2\cdots\Gamma_l^2)\\ &\quad= 2^{l/2}(l-1)!!\sum_{i_1,j_1,k_1,\ldots,k_{l/2}\text{ all distinct}} E(\Gamma_1^2)\cdots E(\Gamma_l^2)+O(n^{3l/2-1})\\ &\quad= 2^{l/2}(l-1)!!n(n-1)\cdots(n-3l/2+1)(\sigma_n^2)^l+O(n^{3l/2-1}), \end{aligned} \tag{80}$$

where the second equality invokes Lemma 3. Here, for notational simplicity, $\Gamma_p, p=1,\ldots,l$ denotes one arbitrary off-diagonal entry in $\Gamma$. Eq. (78), Eq. (79) and Eq. (80) together yield

$$\begin{aligned} E(M_n^l) &= \frac{1}{N^l}\left\{2^{l/2}(l-1)!!n(n-1)\cdots(n-3l/2+1)(\sigma_n^2)^l+O(n^{3l/2-1})\right\}\\ &= (\widetilde{\sigma}_n^2)^{l/2}(l-1)!!+O(n^{-l/2-1}). \end{aligned} \tag{81}$$

Next, when $l$ is odd, per the previous discussion, we can conduct $(1,2)$ actions at most $(l-1)/2$ times on $l$ separate chains. Thus,

$$\max_{t,r_1,\ldots,r_t} n^{l+\sum_{i=1}^t r_i} = O(n^{3l/2-1/2}),$$

and

$$E(M_n^l) = \frac{1}{N^l}\times O(n^{3l/2-1/2}) = O(n^{-l/2-1/2}). \tag{82}$$

So, by combining Eq. (81) and Eq. (82), we have established that

$$\lim_{n\to\infty} E\left(\widetilde{\sigma}_n^{-1} M_n\right)^l = \begin{cases} (l-1)!! & \text{when } l \text{ is even,} \\ 0 & \text{when } l \text{ is odd.} \end{cases}$$

In particular, the above moment quantities are exactly those for the standard normal distribution. Hence, from Billingsley (1995, Theorem 30.1 and Theorem 30.2), as $n \to \infty$,

$$\widetilde{\sigma}_n^{-1} M_n \to N(0,1) \qquad \text{in distribution.}$$

This completes the proof of Lemma 8. □

## References


Athreya, A., Cape, J. & Tang, M. (2022). Eigenvalues of stochastic blockmodel graphs and random graphs with low-rank edge probability matrices. *Sankhya A* **84**, 36–63.

Bai, Z. & Silverstein, J. W. (2010). *Spectral analysis of large dimensional random matrices*. Springer.

Bai, Z. D. & Yin, Y. Q. (1988). Necessary and sufficient conditions for almost sure convergence of the largest eigenvalue of a Wigner matrix. *Annals of Probability* **16**, 1729–1741.

Billingsley, P. (1995). *Probability and measure*. Wiley Series in Probability and Statistics. Wiley.

Billingsley, P. (2013). *Convergence of probability measures*. John Wiley & Sons.

Cape, J., Yu, X. & Liao, J. Z. (2024). Robust spectral clustering with rank statistics. *Journal of Machine Learning Research* **25**, 1–81.

Chen, Y., Chi, Y., Fan, J. & Ma, C. (2021). Spectral methods for data science: a statistical perspective. *Foundations and Trends® in Machine Learning* **14**, 1–246.

Fan, J., Fan, Y., Han, X. & Lv, J. (2022). Asymptotic theory of eigenvectors for random matrices with diverging spikes. *Journal of the American Statistical Association* **117**, 996–1009.

Füredi, Z. & Komlós, J. (1981). The eigenvalues of random symmetric matrices. *Combinatorica* **1**, 233–241.

Hájek, J. (1968). Asymptotic normality of simple linear rank statistics under alternatives. *Annals of Mathematical Statistics* **39**, 325–346.

Marchal, O. & Arbel, J. (2017). On the sub-Gaussianity of the Beta and Dirichlet distributions. *Electronic Communications in Probability* **22**, 1–14.

Vershynin, R. (2018). *High-dimensional probability: an introduction with applications in data science*, vol. 47. Cambridge University Press.

Yu, Y., Wang, T. & Samworth, R. J. (2015). A useful variant of the Davis–Kahan theorem for statisticians. *Biometrika* **102**, 315–323.
